# Supplementary material for: On Measuring Fairness in Generative Models
Source: arXiv:2310.19297 source file (2023-10-30)
Supplement: Supplementary file 1 [file Appendix.tex]

\newpage
This supplementary provides additional details and experiments to further support our 
proposed 
CLassifier
Error-Aware Measurement (CLEAM) for fairness measurement
of generative models.
{\bf Program code has been submitted as part of the supplementary materials}.
The supplementary materials are organised as the following:
\begin{itemize}
    \item Section A: Related Work
    \begin{itemize}
        \item A.1: Fairness in Classifier vs Generative Models
        \item A.2: CLEAM versus Other Calibration Techniques
    \end{itemize}
    \item Section B: Details on Modelling 
    \begin{itemize}
        \item B.1: Details of Theoretical Modelling 
        \item B.2: Additional Details on CLEAM Algorithm
    \end{itemize}
    \item Section C: Validating Proposed Model's Accuracy
    \begin{itemize}
        \item C.1: Validation of Sample-Based Estimate vs Model-Based Estimate
        \item C.2: Goodness-Of-Fit Test: $\phat$ from the Real GAN in \cite{choiFairGenerativeModeling2020a} with Our Theoretical Model
    \end{itemize}
    \item Section D: Hyper-Parameter Settings in our Experiments
    \item Section E: Additional Analysis
    \begin{itemize}
        \item E.1: Retraining VGG-16 for Diversity\cite{keswaniAuditingDiversityUsing2021} Measures
        \item E.2: Results of Proposed CLEAM on Different LA ($\texttt{Young}, \texttt{Attractive}$)
        \item E.3: Results of Proposed CLEAM with Different LA Classifiers (MobileNetV2 \cite{sandlerMobileNetV2InvertedResiduals2018})
        \item E.4: Results of Proposed CLEAM with Different FD Measures
        \item E.5: Analysing CLEAM on MaGNET \cite{humayunMaGNETUniformSampling2021a}
        \item E.6: Validating CLEAM for the Real GANs in \cite{choiFairGenerativeModeling2020a} Using Manually Labelled Samples
    \end{itemize}
    \item Section F: Limitations
    
\end{itemize}
\newpage
\section{Related Work}
\subsection{Fairness in Classifiers vs Generative models}
{\bf Fairness in Generative Models.}
Fairness in machine learning (ML) is mostly studied for the classification problem, where generally the objective is to handle a classification task independent of a sensitive LA in the input data (\eg making `hiring' decisions independent of \texttt{Gender}). Different measurement metrics are used for this objective including well-known Equalised Odds, Equalised Opportunity \cite{hardtEqualityOpportunitySupervised2016} and Demographic Parity \cite{feldmanCertifyingRemovingDisparate2015}. However, the definition of fairness is quite different for generative models: equal generation probability w.r.t a specific LA. For example,  for LA \texttt{Gender}, in a batch of generated images with a fair generator,  the number of {\em male} and {\em female} images are expected to be same.
Because of this difference in the definition, the conventional fairness metrics used for classification cannot be applied to generative models. As such, usually, the problem of measuring fairness in generative models is transformed into measuring the similarity between the probability distribution of the generated sample \wrt a LA ($\pstar$) and a target distribution $\pbar$, which usually is a uniform distribution \cite{choiFairGenerativeModeling2020a,tanImprovingFairnessDeep2020,frankelFairGenerationPrior2020}. 
Note that since the distribution of the LA in generated samples ($\pstar$) is unknown, an additional classifier is used to estimate it. Due to the inaccuracy in the classifier, it's estimated value $\phat$ is usually different from the $\pstar$, and the large differences can make the measurement system unreliable.

\section{Details on Modelling}
\subsection{Details of Theoretical Modelling }
As discussed, we model our CLEAM framework, in terms of a multinomial distribution, $N_{\bC}\sim Multinormial(n,\bp)$.
\begin{equation*}
    \bC=
    \begin{bmatrix}
        C_{0|0}\\
        C_{1|0}\\
        C_{1|1}\\
        C_{0|1}\\     
    \end{bmatrix}
    \bp=
    \begin{bmatrix}
        \pstar_0\alpha_0\\
        \pstar_0\alpha_0'\\
        \pstar_1\alpha_1\\
        \pstar_1\alpha_1'\\     
    \end{bmatrix}
\end{equation*}
\textbf{Assumptions:} 
\begin{enumerate}
    \item \textbf{Classifiers are reasonably accurate.} We state that, given the advancement in classifiers architecture, and the assumption that the classifier is trained with proper training procedures, it is a reasonable assumption that it achieves reasonable accuracy and hence, $\alpha_0\neq0$ and $\alpha_1\neq0$. Similarly, we assume that it is highly unlikely to have a perfect classifier and as such $\alpha'_0\neq0$ and $\alpha'_1\neq0$.  
    \item \textbf{Generators are not completely biased.} Given that a generator is trained on a reliable dataset with the availability of all classes of a given LA, coupled with the advancement in generator's architecture, it is a fair assumption that the generator would learn some representation of each LA and not be completely biased, as such $\pstar_0\neq0$ and $\pstar_1\neq0$.
\end{enumerate}
Given that $\pstar_i,\alpha_i,\alpha'_i \neq 0,\; \forall i\in\{0,1\}$, then $0<\bp<1$ and is not near the boundaries of the parameter space. Hence, we can approximate the multinormial distribution as a Gaussian, $N_{\bC}\sim\mathcal{N}(n\bp,n\bM)$.
\begin{equation*}
    \bM=
        \begin{bmatrix}
        \pstar_0\alpha_0 & 0 & 0 & 0\\
        0 & \pstar_0\alpha_0' & 0 & 0\\
        0 & 0 & \pstar_1\alpha_1 & 0\\
        0 & 0 & 0 &  \pstar_1\alpha_1'\\ 
    \end{bmatrix}
    -
        \begin{bmatrix}
        (\pstar_0\alpha_0)^2 & {(\pstar_0)}^2\alpha_0\alpha_0' & \pstar_0\pstar_1\alpha_0\alpha_1 & \pstar_0\pstar_1\alpha_0\alpha_1'
        \\
        {(\pstar_0})^2\alpha_0\alpha_0' & (\pstar_0\alpha_0')^2  & \pstar_0\pstar_1\alpha_0'\alpha_1 & \pstar_0\pstar_1\alpha_0'\alpha_1'
        \\
        \pstar_0\pstar_1\alpha_0\alpha_1 & \pstar_0\pstar_1\alpha_0'\alpha_1 & (\pstar_1\alpha_1)^2 & (\pstar_1)^2\alpha_1\alpha_1'
        \\
        \pstar_0\pstar_1\alpha_0\alpha_1' & \pstar_0\pstar_1\alpha_0'\alpha_1' & (\pstar_1)^2\alpha_1\alpha_1' & (\pstar_1\alpha_1')^2\\ 
    \end{bmatrix}
\end{equation*}
with that, we solve for the marginal distribution of $N_{C_{0}}$ and $N_{C_{1}}$
\begin{gather*}
%\begin{equation*}
%    \begin{aligned}
    N_{C_0}=N_{C_{0|0}}+N_{C_{0|1}}\sim \mathcal{N}(\Tilde{\mu}_{C_0},\Tilde{\sigma}^2_{C_0})\\
    \Tilde{\mu}_{C_0}=n(\pstar_0\alpha_0+\pstar_1\alpha_1')\\
    \Tilde{\sigma}^2_{C_0}=n(\pstar_0\alpha_0-(\pstar_0\alpha_0)^2)+n(\pstar_1\alpha_1'-(\pstar_1\alpha_1')^2)
    + 2 {n\pstar_0\pstar_1\alpha_0\alpha_1'}
    %\sqrt{n(\pstar_0\alpha_0-(\pstar_0\alpha_0)^2)}\sqrt{n(\pstar_1\alpha_1'-(\pstar_1\alpha_1')^2})
%    \end{aligned}
%\end{equation*}
\end{gather*}
\begin{gather*}
%\begin{equation*}
%    \begin{aligned}
    N_{C_1}=N_{C_{1|0}}+N_{C_{1|1}}\sim \mathcal{N}(\Tilde{\mu}_{C_1},\Tilde{\sigma}^2_{C_1})\\
    \Tilde{\mu}_{C_1}=n(\pstar_0\alpha_0'+\pstar_1\alpha_1)\\
    \Tilde{\sigma}^2_{C_1}=n(\pstar_0\alpha_0'-(\pstar_0\alpha_0')^2)+n(\pstar_1\alpha_1-(\pstar_1\alpha_1)^2)
    +2{n\pstar_0\pstar_1\alpha_0'\alpha_1}
    %\sqrt{n(\pstar_0\alpha_0'-(\pstar_0\alpha_0')^2)}\sqrt{n(\pstar_1\alpha_1+(\pstar_1\alpha_1)^2)}
%    \end{aligned}
%\end{equation*}
\end{gather*}
We then normalise $N_{C_i}$, to get $\phat_i=\frac{1}{n}N_{C_i},\;i\in\{0,1\}$
\begin{gather*}
%\begin{equation*}
%    \begin{aligned}
    \phat_0\sim \mathcal{N}(\Tilde{\mu}_{\phat_0},\Tilde{\sigma}^2_{\phat_0})\\
    \Tilde{\mu}_{\phat_0}=\pstar_0\alpha_0+\pstar_1\alpha_1'\\
    \Tilde{\sigma}^2_{\phat_0}=\frac{1}{n}(\pstar_0\alpha_0-(\pstar_0\alpha_0)^2)+\frac{1}{n}(\pstar_1\alpha_1'-(\pstar_1\alpha_1')^2)
    + \frac{2}{n} {\pstar_0\pstar_1\alpha_0\alpha_1'}
    %\sqrt{n(\pstar_0\alpha_0-(\pstar_0\alpha_0)^2)}\sqrt{n(\pstar_1\alpha_1'-(\pstar_1\alpha_1')^2})
%    \end{aligned}
%\end{equation*}
\end{gather*}
\begin{gather*}
%\begin{equation*}
%    \begin{aligned}
    \phat_1\sim \mathcal{N}(\mu_{\phat_1},\sigma^2_{\phat_1})\\
    \Tilde{\mu}_{\phat_1}=(\pstar_0\alpha_0'+\pstar_1\alpha_1)\\
    \Tilde{\sigma}^2_{\phat_1}=\frac{1}{n}(\pstar_0\alpha_0'-(\pstar_0\alpha_0')^2)+\frac{1}{n}(\pstar_1\alpha_1-(\pstar_1\alpha_1)^2)
    +\frac{2}{n}{\pstar_0\pstar_1\alpha_0'\alpha_1}
    %\sqrt{n(\pstar_0\alpha_0'-(\pstar_0\alpha_0')^2)}\sqrt{n(\pstar_1\alpha_1+(\pstar_1\alpha_1)^2)}
%    \end{aligned}
%\end{equation*}
\end{gather*}

\FloatBarrier
\subsection{Additional Details on CLEAM Algorithm}
\label{apx:proposedmethod}
In the following, we show that the maximum likelihood estimate (MLE) of the population mean for a Gaussian distribution, is it's sample mean:
%\textcolor{red}{(Could we add some details, \eg, what is this term? whay we are taking the derivative of this \wrt $\hat{\mu}$?)}
\begin{gather*}
%\begin{equation*}
    \label{eqn:MLEAppen}
%    \begin{aligned}
    \frac{\partial}{\partial \Tilde{\mu}_{\phat_0}} \prod_{i=1}^s ln(\frac{1}{\Tilde{\sigma}_{\phat_0} \sqrt{2 \pi}} e^{\frac{-(\hat{p}^i_0 - \Tilde{\mu}_{\phat_0})^2}{2 \Tilde{\sigma}_{\phat_0}^2}})=0\\
    \frac{1}{\Tilde{\sigma}_{\phat_0}^2} \sum_{i=0}^s (\hat{p}^i_0-\Tilde{\mu}_{\phat_0})=0\\ 
    \Tilde{\mu}_{\phat_0}=\frac{1}{s} \sum_i^s \hat{p}^i_0=\Ddot{\mu}_{\phat_0}
%    \end{aligned}
%\end{equation*}
\end{gather*}
This proof shows that, given a Gaussian distribution with population mean $\tilde{\mu}_{\phat_0}$ and standard deviation $\tilde{\sigma}_{\phat_0}$, we can first find the joint probability distribution from the product of each probabilistic outcome (we introduce the natural log as a monotonic function, for ease of calculation). Then, to find the MLE of $\tilde{\mu}_{\phat_0}$, we take the partial derivative of this joint distribution \wrt $\tilde{\mu}_{\phat_0}$, and solve for its the maximum value. We find this maximum value to be equal to the sample mean, $\Ddot{\mu}_{\phat_0}$.

From this, given that $s$ is large, we assume that the sample mean is a good approximation for the population mean and equate them. We then solve for the maximum likelihood point estimate of $\pstar$, which we denoted with $\mu_{\texttt{CLEAM}}(p^*)$.
\begin{gather*}
%\begin{equation*}
%    \begin{aligned}
    \Ddot{\mu}_{\phat_0}=\Tilde{\mu}_{\phat_0}=p^*_0\alpha_{0} + (1-p^*_0)\alpha'_{1}\\
    \mu_{\texttt{CLEAM}}(p^*_0)=\frac{\Ddot{\mu}_{\phat_0}-\alpha'_{1}}{\alpha_0-\alpha'_{1}}=\frac{\Ddot{\mu}_{\phat_0}-1+\alpha_1}{\alpha_0-1+\alpha_1} \\
    \mu_{\texttt{CLEAM}}(p^*_1)=1-\mu_{\texttt{CLEAM}}(p^*_0)
%    \end{aligned}
%\end{equation*}
\end{gather*}
However, we acknowledge that there exist other statistically probable solutions for $p^*$ that could output the $s$ $\phat$ samples, other than the Maximum likelihood point estimate of $p^*$. We thus propose the following approximation for the $95\%$ confidence interval of $p^*$.
Since $\phat$ distribution is assumed Gaussian, we can propose the following equation. Recall that the notations $\Ddot{\mu}_{\phat_0}$ and $\Ddot{\sigma}_{\phat_0}$ are the sample mean and standard deviation respectively.
\begin{equation*}
    \begin{aligned}
    Pr(-z_{\frac{\delta}{2}}\leq \frac{\Ddot{\mu}_{\phat_0}-\Tilde{\mu}_{\phat_0}}{\frac{\Ddot{{\sigma}}_{\phat_0}}{\sqrt{s}}}\leq \z_{\frac{\delta}{2}})=1-\delta
    \quad 
    \\ ,where \quad
    \Ddot{\mu}_{\phat_0}=\frac{1}{s} \sum_i^s \hat{p}^i_0
    \quad and \quad
    \Ddot{\sigma}_{\phat_0}=\sqrt{\frac{\sum^s_{i=1}(\phat^i_0-\Ddot{\mu}_{\phat_0})}{s}}
    \end{aligned}
\end{equation*}
Solving for $\Tilde{\mu}_{\phat}$, we get
\begin{equation*}
    \begin{aligned}
    Pr(-z_{\frac{\delta}{2}}\leq \frac{\Ddot{\mu}_{\phat_0}-\Tilde{\mu}_{\phat_0}}{\frac{\Ddot{\sigma}_{\phat_0}}{\sqrt{s}}}\leq \z_{\frac{\delta}{2}})=1-\delta
    \end{aligned}
\end{equation*}
\begin{equation*}
    \begin{aligned}
    Pr(\Ddot{\mu}_{\phat_0}+z_\frac{\delta}{2}(\frac{\Ddot{\sigma}_{\phat_0}}{\sqrt{s}})\geq \Tilde{\mu}_{\phat_0} \geq \Ddot{\mu}_{\phat_0}- z_{\frac{\alpha}{2}}\frac{\Ddot{\sigma}_{\phat_0}}{\sqrt{s}})=1-\delta
    \end{aligned}
\end{equation*}
Similarly, given that $s$ is large, we approximate $\Tilde{\mu}_{\phat}=\pstar_0\alpha_0+\pstar_1\alpha_1'=\pstar_0(\alpha_0-\alpha_1')+\alpha_1'$. This allows us to formulate the following:
\begin{equation}
    \label{eqn:CIwithsamplestd}
    \begin{aligned}
    Pr(\frac{\Ddot{\mu}_{\phat_0}+z_\frac{\delta}{2}(\frac{\Ddot{\sigma}_{\phat_0}}{\sqrt{s}})-\alpha_1'}{\alpha_0-\alpha_1'}
    \geq 
    \pstar_0
    \geq 
    \frac{\Ddot{\mu}_{\phat_0}- z_{\frac{\alpha}{2}}\frac{\Ddot{\sigma}_{\phat_0}}{\sqrt{s}}-\alpha_1'}{\alpha_0-\alpha_1'})=1-\delta
    \end{aligned}
\end{equation}
As such when $\delta=0.05$, we can determine that the $95\%$ approximated confidence interval of $\pstar_0$ is :
\begin{equation*}
    \begin{aligned}
    \rho_{\texttt{CLEAM}}(\pstar_0)=[\mathcal{L}(\pstar_0),\mathcal{U}(\pstar_0)]=
    [\frac{\Ddot{\mu}_{\phat_0}-1.96(\frac{\Ddot{\sigma}_{\phat_0}}{\sqrt{s}})-\alpha_1'}{\alpha_0-\alpha_1'}
    \quad,\quad
    \frac{\Ddot{\mu}_{\phat_0}+ 1.96\frac{\Ddot{\sigma}_{\phat_0}}{\sqrt{s}}-\alpha_1'}{\alpha_0-\alpha_1'}]
    \end{aligned}
\end{equation*}
\textbf{Alternative solution:} 
As an alternative solution to Eqn. \ref{eqn:CIwithsamplestd}, 
the theoretical standard deviation i.e., $\Tilde{\sigma}_{\phat_0}$, 
could be used, as shown in Eqn. \ref{eqn:CIwithpopstd}. 
But as we will discuss in Sec. \ref{sec:sampleBasedEstimate}, the sample-based estimates and the model-based estimates are very close, and the sample-based estimates can be easily calculated. Therefore,  
we apply the sample-based standard deviation as discussed above.

% in hopes of getting a better approximate. But as seen from the following equation, factorising $\pstar_0$ is difficult. As a result heuristic algorithms are likely to be used, which are computationally inefficient. As such, 

% , since our experiments had shown that the empirical approximation was sufficient and less computationally intensive. 
\begin{equation}
    \label{eqn:CIwithpopstd}
    \begin{aligned}
    Pr(-z_{\frac{\delta}{2}}\leq \frac{\Ddot{\mu}_{\phat_0}-(\pstar_0(\alpha_0-\alpha_1')+\alpha_1')}{\sqrt{\frac{1}{n}(\pstar_0\alpha_0-(\pstar_0\alpha_0)^2)+\frac{1}{n}(\pstar_1\alpha_1'-(\pstar_1\alpha_1')^2)
    + \frac{2}{n} {\pstar_0\pstar_1\alpha_0\alpha_1'}}}\leq z_{\frac{\delta}{2}})=1-\delta
    \end{aligned}
\end{equation}

\subsection{Fairness in Classifiers vs Generative models}
{\bf Fairness in Generative Models.}
Fairness in machine learning (ML) is mostly studied for the classification problem, where generally the objective is to handle a classification task independent of a sensitive LA in the input data (\eg making `hiring' decisions independent of \texttt{Gender}). Different measurement metrics are used for this objective including well-known Equalised Odds, Equalised Opportunity \cite{hardtEqualityOpportunitySupervised2016} and Demographic Parity \cite{feldmanCertifyingRemovingDisparate2015}. However, the definition of fairness is quite different for generative models: equal generation probability w.r.t a specific LA. For example,  for LA \texttt{Gender}, in a batch of generated images with a fair generator,  the number of {\em male} and {\em female} images are expected to be same.
Because of this difference in the definition, the conventional fairness metrics used for classification cannot be applied to generative models. As such, usually, the problem of measuring fairness in generative models is transformed into measuring the similarity between the probability distribution of the generated sample \wrt a LA ($\pstar$) and a target distribution $\pbar$, which usually is a uniform distribution \cite{choiFairGenerativeModeling2020a,tanImprovingFairnessDeep2020,frankelFairGenerationPrior2020}. 
Note that since the distribution of the LA in generated samples ($\pstar$) is unknown, an additional classifier is used to estimate it. Due to the inaccuracy in the classifier, it's estimated value $\phat$ is usually different from the $\pstar$, and the large differences can make the measurement system unreliable.

\subsection{CLEAM versus Other Calibration Techniques}
Conventional classifier calibration methods usually work on soft labels (probabilities). Note that in our framework, a threshold is applied to the output probabilities to determine the hard label. %In our application, regular classifier calibration does not affect the hard label that much. 
Therefore, in our application that deals with hard labels, regular classification techniques are less effective.
To investigate this, we conduct a few calibration experiment by applying some popular classifier calibration techniques; temperature scaling(T-scaling) \cite{guoCalibrationModernNeural2017}, Isotonic Regression\cite{nyberg2021reliably} and Platt Scaling\cite{platt1999probabilistic}  on a pre-trained ResNet-18\cite{heDeepResidualLearning2016} LA classifier. In Fig. \ref{fig:Calibration_curve}, we see that T-scaling is the most effective in correcting the calibration curve to the ideal Ref line.  
Note that, this Ref line indicates that the classifier is perfectly calibrated \wrt the soft labels.
%However, as shown in Fig. \ref{fig:Calibration_Error} T-scaling shows negligible improvement in normalized error, demonstraing that traditional calibration technique may not have a direct correlation to hard label calibration, which CLEAM aims to address.
\begin{figure}[h]
    \centering
    \includegraphics[scale=0.5]{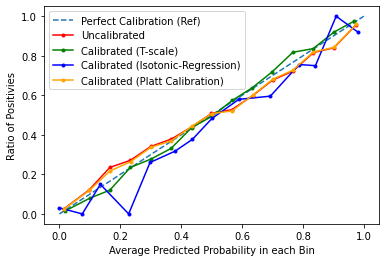}
    \caption{Calibration Curve on ResNet-18 and LA $\texttt{Attractive}$. We observe that the T-scaling is the most effective technique in improving soft label calibration and Isotonic regression the worst. However, this same trend does not follow in the hard label errors of Fig \ref{fig:Calibration_Error}.}
    \label{fig:Calibration_curve}
\end{figure}

\label{sub:traditionalCalibration}
\begin{figure}[!h]
    \centering
    \includegraphics[scale=0.4]{Figures/Calibration/Calibration_Effectiveness.pdf}
    \caption{\textbf{Comparing Calibration Techniques}: Using the pseudo-generator, we compare CLEAM against well known calibration techniques, overall we observe that previous techniques are significantly less effective, achieving an average error of; T-Scaling: $12.4\%$, Isotonic Regression: $10.1\%$, Platt Calibration: $14.5\%$ and uncalibrated (baseline): $12.4\%$ against CLEAM: $2.0\%$ }
    \label{fig:Calibration_Error}
\end{figure}
Next, using the pseudo-generator from Sec. 5 of the main paper, we utilised the calibrated classifiers earlier and compare them against CLEAM (which was applied on an uncalibrated model).
%against the other well known calibration techniques.
%, namely T-scaling, Isotonic regression and Platt Scaling \cite{guoCalibrationModernNeural2017}. 
\textbf{In our results,} seen in Fig. \ref{fig:Calibration_Error}, we observe that these traditional calibration methods are less effective in correcting the LA distribution error. 
In fact, methods like Platt scaling worsen the error, and T scaling ---which is shown in \cite{guoCalibrationModernNeural2017} and our experiment to be one of the most effective traditional calibration methods--- does not change class predictions (hard labels), but merely perturb the soft labels. 
This demonstrates that traditional calibration technique may not have a direct correlation to hard label calibration, which CLEAM aims to address.

\FloatBarrier
\clearpage
\section{Details on Modelling}
\subsection{Details of Theoretical Modelling }
As discussed, we model our CLEAM framework, in terms of a multinomial distribution, $N_{\bC}\sim Multinormial(n,\bp)$.
\begin{equation*}
    \bC=
    \begin{bmatrix}
        C_{0|0}\\
        C_{1|0}\\
        C_{1|1}\\
        C_{0|1}\\     
    \end{bmatrix}
    \bp=
    \begin{bmatrix}
        \pstar_0\alpha_0\\
        \pstar_0\alpha_0'\\
        \pstar_1\alpha_1\\
        \pstar_1\alpha_1'\\     
    \end{bmatrix}
\end{equation*}
\textbf{Assumptions:} 
\begin{enumerate}
    \item \textbf{Classifiers are reasonably accurate.} We state that, given the advancement in classifiers architecture, and the assumption that the classifier is trained with proper training procedures, it is a reasonable assumption that it achieves reasonable accuracy and hence, $\alpha_0\neq0$ and $\alpha_1\neq0$. Similarly, we assume that it is highly unlikely to have a perfect classifier and as such $\alpha'_0\neq0$ and $\alpha'_1\neq0$.  
    \item \textbf{Generators are not completely biased.} Given that a generator is trained on a reliable dataset with the availability of all classes of a given LA, coupled with the advancement in generator's architecture, it is a fair assumption that the generator would learn some representation of each LA and not be completely biased, as such $\pstar_0\neq0$ and $\pstar_1\neq0$.
\end{enumerate}
Given that $\pstar_i,\alpha_i,\alpha'_i \neq 0,\; \forall i\in\{0,1\}$, then $0<\bp<1$ and is not near the boundaries of the parameter space. Hence, we can approximate the multinormial distribution as a Gaussian, $N_{\bC}\sim\mathcal{N}(n\bp,n\bM)$.
\begin{equation*}
    \bM=
        \begin{bmatrix}
        \pstar_0\alpha_0 & 0 & 0 & 0\\
        0 & \pstar_0\alpha_0' & 0 & 0\\
        0 & 0 & \pstar_1\alpha_1 & 0\\
        0 & 0 & 0 &  \pstar_1\alpha_1'\\ 
    \end{bmatrix}
    -
        \begin{bmatrix}
        (\pstar_0\alpha_0)^2 & {(\pstar_0)}^2\alpha_0\alpha_0' & \pstar_0\pstar_1\alpha_0\alpha_1 & \pstar_0\pstar_1\alpha_0\alpha_1'
        \\
        {(\pstar_0})^2\alpha_0\alpha_0' & (\pstar_0\alpha_0')^2  & \pstar_0\pstar_1\alpha_0'\alpha_1 & \pstar_0\pstar_1\alpha_0'\alpha_1'
        \\
        \pstar_0\pstar_1\alpha_0\alpha_1 & \pstar_0\pstar_1\alpha_0'\alpha_1 & (\pstar_1\alpha_1)^2 & (\pstar_1)^2\alpha_1\alpha_1'
        \\
        \pstar_0\pstar_1\alpha_0\alpha_1' & \pstar_0\pstar_1\alpha_0'\alpha_1' & (\pstar_1)^2\alpha_1\alpha_1' & (\pstar_1\alpha_1')^2\\ 
    \end{bmatrix}
\end{equation*}
with that, we solve for the marginal distribution of $N_{C_{0}}$ and $N_{C_{1}}$
\begin{gather*}
%\begin{equation*}
%    \begin{aligned}
    N_{C_0}=N_{C_{0|0}}+N_{C_{0|1}}\sim \mathcal{N}(\Tilde{\mu}_{C_0},\Tilde{\sigma}^2_{C_0})\\
    \Tilde{\mu}_{C_0}=n(\pstar_0\alpha_0+\pstar_1\alpha_1')\\
    \Tilde{\sigma}^2_{C_0}=n(\pstar_0\alpha_0-(\pstar_0\alpha_0)^2)+n(\pstar_1\alpha_1'-(\pstar_1\alpha_1')^2)
    + 2 {n\pstar_0\pstar_1\alpha_0\alpha_1'}
    %\sqrt{n(\pstar_0\alpha_0-(\pstar_0\alpha_0)^2)}\sqrt{n(\pstar_1\alpha_1'-(\pstar_1\alpha_1')^2})
%    \end{aligned}
%\end{equation*}
\end{gather*}
\begin{gather*}
%\begin{equation*}
%    \begin{aligned}
    N_{C_1}=N_{C_{1|0}}+N_{C_{1|1}}\sim \mathcal{N}(\Tilde{\mu}_{C_1},\Tilde{\sigma}^2_{C_1})\\
    \Tilde{\mu}_{C_1}=n(\pstar_0\alpha_0'+\pstar_1\alpha_1)\\
    \Tilde{\sigma}^2_{C_1}=n(\pstar_0\alpha_0'-(\pstar_0\alpha_0')^2)+n(\pstar_1\alpha_1-(\pstar_1\alpha_1)^2)
    +2{n\pstar_0\pstar_1\alpha_0'\alpha_1}
    %\sqrt{n(\pstar_0\alpha_0'-(\pstar_0\alpha_0')^2)}\sqrt{n(\pstar_1\alpha_1+(\pstar_1\alpha_1)^2)}
%    \end{aligned}
%\end{equation*}
\end{gather*}
We then normalise $N_{C_i}$, to get $\phat_i=\frac{1}{n}N_{C_i},\;i\in\{0,1\}$
\begin{gather*}
%\begin{equation*}
%    \begin{aligned}
    \phat_0\sim \mathcal{N}(\Tilde{\mu}_{\phat_0},\Tilde{\sigma}^2_{\phat_0})\\
    \Tilde{\mu}_{\phat_0}=\pstar_0\alpha_0+\pstar_1\alpha_1'\\
    \Tilde{\sigma}^2_{\phat_0}=\frac{1}{n}(\pstar_0\alpha_0-(\pstar_0\alpha_0)^2)+\frac{1}{n}(\pstar_1\alpha_1'-(\pstar_1\alpha_1')^2)
    + \frac{2}{n} {\pstar_0\pstar_1\alpha_0\alpha_1'}
    %\sqrt{n(\pstar_0\alpha_0-(\pstar_0\alpha_0)^2)}\sqrt{n(\pstar_1\alpha_1'-(\pstar_1\alpha_1')^2})
%    \end{aligned}
%\end{equation*}
\end{gather*}
\begin{gather*}
%\begin{equation*}
%    \begin{aligned}
    \phat_1\sim \mathcal{N}(\mu_{\phat_1},\sigma^2_{\phat_1})\\
    \Tilde{\mu}_{\phat_1}=(\pstar_0\alpha_0'+\pstar_1\alpha_1)\\
    \Tilde{\sigma}^2_{\phat_1}=\frac{1}{n}(\pstar_0\alpha_0'-(\pstar_0\alpha_0')^2)+\frac{1}{n}(\pstar_1\alpha_1-(\pstar_1\alpha_1)^2)
    +\frac{2}{n}{\pstar_0\pstar_1\alpha_0'\alpha_1}
    %\sqrt{n(\pstar_0\alpha_0'-(\pstar_0\alpha_0')^2)}\sqrt{n(\pstar_1\alpha_1+(\pstar_1\alpha_1)^2)}
%    \end{aligned}
%\end{equation*}
\end{gather*}

\FloatBarrier
\subsection{Additional Details on CLEAM Algorithm}
\label{apx:proposedmethod}
In the following, we show that the maximum likelihood estimate (MLE) of the population mean for a Gaussian distribution, is it's sample mean:
%\textcolor{red}{(Could we add some details, \eg, what is this term? whay we are taking the derivative of this \wrt $\hat{\mu}$?)}
\begin{gather*}
%\begin{equation*}
    \label{eqn:MLEAppen}
%    \begin{aligned}
    \frac{\partial}{\partial \Tilde{\mu}_{\phat_0}} \prod_{i=1}^s ln(\frac{1}{\Tilde{\sigma}_{\phat_0} \sqrt{2 \pi}} e^{\frac{-(\hat{p}^i_0 - \Tilde{\mu}_{\phat_0})^2}{2 \Tilde{\sigma}_{\phat_0}^2}})=0\\
    \frac{1}{\Tilde{\sigma}_{\phat_0}^2} \sum_{i=0}^s (\hat{p}^i_0-\Tilde{\mu}_{\phat_0})=0\\ 
    \Tilde{\mu}_{\phat_0}=\frac{1}{s} \sum_i^s \hat{p}^i_0=\Ddot{\mu}_{\phat_0}
%    \end{aligned}
%\end{equation*}
\end{gather*}
This proof shows that, given a Gaussian distribution with population mean $\tilde{\mu}_{\phat_0}$ and standard deviation $\tilde{\sigma}_{\phat_0}$, we can first find the joint probability distribution from the product of each probabilistic outcome (we introduce the natural log as a monotonic function, for ease of calculation). Then, to find the MLE of $\tilde{\mu}_{\phat_0}$, we take the partial derivative of this joint distribution \wrt $\tilde{\mu}_{\phat_0}$, and solve for its the maximum value. We find this maximum value to be equal to the sample mean, $\Ddot{\mu}_{\phat_0}$.

From this, given that $s$ is large, we assume that the sample mean is a good approximation for the population mean and equate them. We then solve for the maximum likelihood point estimate of $\pstar$, which we denoted with $\mu_{\texttt{CLEAM}}(p^*)$.
\begin{gather*}
%\begin{equation*}
%    \begin{aligned}
    \Ddot{\mu}_{\phat_0}=\Tilde{\mu}_{\phat_0}=p^*_0\alpha_{0} + (1-p^*_0)\alpha'_{1}\\
    \mu_{\texttt{CLEAM}}(p^*_0)=\frac{\Ddot{\mu}_{\phat_0}-\alpha'_{1}}{\alpha_0-\alpha'_{1}}=\frac{\Ddot{\mu}_{\phat_0}-1+\alpha_1}{\alpha_0-1+\alpha_1} \\
    \mu_{\texttt{CLEAM}}(p^*_1)=1-\mu_{\texttt{CLEAM}}(p^*_0)
%    \end{aligned}
%\end{equation*}
\end{gather*}
However, we acknowledge that there exist other statistically probable solutions for $p^*$ that could output the $s$ $\phat$ samples, other than the Maximum likelihood point estimate of $p^*$. We thus propose the following approximation for the $95\%$ confidence interval of $p^*$.
Since $\phat$ distribution is assumed Gaussian, we can propose the following equation. Recall that the notations $\Ddot{\mu}_{\phat_0}$ and $\Ddot{\sigma}_{\phat_0}$ are the sample mean and standard deviation respectively.
\begin{equation*}
    \begin{aligned}
    Pr(-z_{\frac{\delta}{2}}\leq \frac{\Ddot{\mu}_{\phat_0}-\Tilde{\mu}_{\phat_0}}{\frac{\Ddot{{\sigma}}_{\phat_0}}{\sqrt{s}}}\leq \z_{\frac{\delta}{2}})=1-\delta
    \quad 
    \\ ,where \quad
    \Ddot{\mu}_{\phat_0}=\frac{1}{s} \sum_i^s \hat{p}^i_0
    \quad and \quad
    \Ddot{\sigma}_{\phat_0}=\sqrt{\frac{\sum^s_{i=1}(\phat^i_0-\Ddot{\mu}_{\phat_0})}{s}}
    \end{aligned}
\end{equation*}
Solving for $\Tilde{\mu}_{\phat}$, we get
\begin{equation*}
    \begin{aligned}
    Pr(-z_{\frac{\delta}{2}}\leq \frac{\Ddot{\mu}_{\phat_0}-\Tilde{\mu}_{\phat_0}}{\frac{\Ddot{\sigma}_{\phat_0}}{\sqrt{s}}}\leq \z_{\frac{\delta}{2}})=1-\delta
    \end{aligned}
\end{equation*}
\begin{equation*}
    \begin{aligned}
    Pr(\Ddot{\mu}_{\phat_0}+z_\frac{\delta}{2}(\frac{\Ddot{\sigma}_{\phat_0}}{\sqrt{s}})\geq \Tilde{\mu}_{\phat_0} \geq \Ddot{\mu}_{\phat_0}- z_{\frac{\alpha}{2}}\frac{\Ddot{\sigma}_{\phat_0}}{\sqrt{s}})=1-\delta
    \end{aligned}
\end{equation*}
Similarly, given that $s$ is large, we approximate $\Tilde{\mu}_{\phat}=\pstar_0\alpha_0+\pstar_1\alpha_1'=\pstar_0(\alpha_0-\alpha_1')+\alpha_1'$. This allows us to formulate the following:
\begin{equation}
    \label{eqn:CIwithsamplestd}
    \begin{aligned}
    Pr(\frac{\Ddot{\mu}_{\phat_0}+z_\frac{\delta}{2}(\frac{\Ddot{\sigma}_{\phat_0}}{\sqrt{s}})-\alpha_1'}{\alpha_0-\alpha_1'}
    \geq 
    \pstar_0
    \geq 
    \frac{\Ddot{\mu}_{\phat_0}- z_{\frac{\alpha}{2}}\frac{\Ddot{\sigma}_{\phat_0}}{\sqrt{s}}-\alpha_1'}{\alpha_0-\alpha_1'})=1-\delta
    \end{aligned}
\end{equation}
As such when $\delta=0.05$, we can determine that the $95\%$ approximated confidence interval of $\pstar_0$ is :
\begin{equation*}
    \begin{aligned}
    \rho_{\texttt{CLEAM}}(\pstar_0)=[\mathcal{L}(\pstar_0),\mathcal{U}(\pstar_0)]=
    [\frac{\Ddot{\mu}_{\phat_0}-1.96(\frac{\Ddot{\sigma}_{\phat_0}}{\sqrt{s}})-\alpha_1'}{\alpha_0-\alpha_1'}
    \quad,\quad
    \frac{\Ddot{\mu}_{\phat_0}+ 1.96\frac{\Ddot{\sigma}_{\phat_0}}{\sqrt{s}}-\alpha_1'}{\alpha_0-\alpha_1'}]
    \end{aligned}
\end{equation*}
\textbf{Alternative solution:} 
As an alternative solution to Eqn. \ref{eqn:CIwithsamplestd}, 
the theoretical standard deviation i.e., $\Tilde{\sigma}_{\phat_0}$, 
could be used, as shown in Eqn. \ref{eqn:CIwithpopstd}. 
But as we will discuss in Sec. \ref{sec:sampleBasedEstimate}, the sample-based estimates and the model-based estimates are very close, and the sample-based estimates can be easily calculated. Therefore,  
we apply the sample-based standard deviation as discussed above.

% in hopes of getting a better approximate. But as seen from the following equation, factorising $\pstar_0$ is difficult. As a result heuristic algorithms are likely to be used, which are computationally inefficient. As such, 

% , since our experiments had shown that the empirical approximation was sufficient and less computationally intensive. 
\begin{equation}
    \label{eqn:CIwithpopstd}
    \begin{aligned}
    Pr(-z_{\frac{\delta}{2}}\leq \frac{\Ddot{\mu}_{\phat_0}-(\pstar_0(\alpha_0-\alpha_1')+\alpha_1')}{\sqrt{\frac{1}{n}(\pstar_0\alpha_0-(\pstar_0\alpha_0)^2)+\frac{1}{n}(\pstar_1\alpha_1'-(\pstar_1\alpha_1')^2)
    + \frac{2}{n} {\pstar_0\pstar_1\alpha_0\alpha_1'}}}\leq z_{\frac{\delta}{2}})=1-\delta
    \end{aligned}
\end{equation}
%man_24nov: is it the ``alternative solution'', maybe you can use eqn number to indicate, it takes a while to figure out
%Chris: Noted and amended.

\FloatBarrier
\clearpage
\section{Validating Proposed Model's Accuracy}
\subsection{ Validation of sample-based Estimate vs Model-Based Estimate}
\label{sec:sampleBasedEstimate}
As described in Sec. 5 of the main paper, we utilise the sample-based estimate, $\Ddot{\mu}_{\phat_0}$,  ${\Ddot{\sigma}^2_{\phat_0}}$ as an approximate for the model-based estimate $\Tilde{\mu}_{\phat_0}$,  ${\Tilde{\sigma}^2_{\phat_0}}$. 
As discussed in the \ref{apx:proposedmethod}, $\Ddot{\mu}_{\phat_0}$ allows us to find the maximum likelihood approximate of $\pstar$ and ${\Ddot{\sigma}^2_{\phat_0}}$ allows us to ease computation.

\textit{\bf To validate this approximation, } we use a batch-size $s=30$ and sample size $n=1k$ in each batch to generate s different $\phat$ values from the pseudo-generators (Sec. 3 of the main paper) with different GT $\pstar$. Then we calculate the sample-based estimates as given in Eqn. (5) and (6) of the main paper. As the GT $\pstar$ is known, we also calculate the model-based estimates as given in Eqn. (3) and (4) of the main paper and compare it against the sample-based estimates.

\textit{\bf Our results} in Tab. \ref{tab:theoreticaleval} shows that both the sample and theoretical means and standard deviations are close approximate to one another. Thus, we can utilise the sample statistics as a close approximation in our proposed method, CLEAM.

Additional results for different values of batch-sizes ($s$) and sample-sizes ($n$) are tabulated in Tab. \ref{tab:theoreticalevals20n1k} and \ref{tab:theoreticalevals30n500}.
Notice that a reduction in $s$ and $n$ values contributed to increased errors between the sample-based and model-based estimates.
 
\begin{table}[!h]
    \centering
    \caption{
        \textbf{Comparing sample-based estimates ($\Ddot{\boldsymbol\mu}_{\boldsymbol\phat_0}$, $\Ddot{\boldsymbol\sigma}_{\boldsymbol\phat_0}$) against model-based estimates ($\tilde{\boldsymbol\mu}_{\boldsymbol\phat_0}$, $\tilde{\boldsymbol\sigma}_{\boldsymbol\phat_0}$).}
        %Validation of using sample-based estimates as given in Eqn. (5) and (6)  in place of model-based estimates as given in Eqn. (3) and (4) of the main paper, using samples from Pseudo Generators with different GT $\pstar$. Number of $\phat $ samples $s=30$ and number of images per batch $n=1k$. The GT $\pstar$ are used to compute the model-based estimates following Eqn. (3) and (4). As $\pstar$ is unknown in practice, we instead use sample-based estimates in our method. 
        The results show that sample-based estimates are close to 
        model-based estimates. 
        Furthermore, note the discrepancy between $p^*_0$ and $\Ddot{\mu}_{\phat_0}$,
        and that between $p^*_0$ and
        $\Tilde{\mu}_{\phat_0}$, highlighting the issue of using $\phat_0$ directly
        to estimate $p^*_0$
        and the
        need to compensate for classifier error as we discussed.
        }
    \resizebox{8.0cm}{!}{
    \begin{tabular}{c @{\hspace{2em}} c @{\hspace{0.1 em}} c @{\hspace{2em}} c @{\hspace{0.1em}} c}
        
        %GT & Mean $\hat{p}_0$ & Std $\hat{p}_0$ & Mean $\hat{p}_0$ &  Std $\hat{p}_0$ \\
      
        \toprule
        GT & \multicolumn{2}{c}{Sampled-based estimates} & \multicolumn{2}{c}{Model-based estimates}
        \\\cmidrule(lr){1-1} \cmidrule(lr){2-3} \cmidrule(lr){4-5} 
        &$\Ddot{\mu}_{\phat_0}$ & $\sqrt{\Ddot{\sigma}^2_{\phat_0}}$ & $\Tilde{\mu}_{\phat_0}$ &  $\sqrt{\Tilde{\sigma}^2_{\phat_0}}$ \\
        
        \midrule
        \multicolumn{5}{c}{Gender, $\balpha$=[0.976,0.979]}\\
        \midrule
        $p^*_0=0.9$ &0.881 & 0.0101 & 0.881  & 0.0106\\
        $p^*_0=0.8$ &0.781 & 0.0133 & 0.785   & 0.0135\\
        $p^*_0=0.7$ &0.692 & 0.0149 & 0.690 & 0.0152\\
        $p^*_0=0.6$ &0.590 & 0.0165 & 0.594   & 0.0162\\
        $p^*_0=0.5$ &0.503 & 0.0164 & 0.499   & 0.0164\\
        \midrule
        \multicolumn{5}{c}{$\balpha$=[0.881,0.887], Black-Hair}\\
        \midrule
        $p^*_0=0.9$ &0.802 & 0.0130 & 0.804  &	0.0139\\
        $p^*_0=0.8$ &0.723 & 0.0151 & 0.727  &	0.0162\\
        $p^*_0=0.7$ &0.653 & 0.0169 & 0.650 &	0.0177\\
        $p^*_0=0.6$ &0.580 & 0.0180 & 0.574   & 0.0186\\
        $p^*_0=0.5$ &0.502 & 0.0180 & 0.497  &	0.0189

    \end{tabular}}
    \label{tab:theoreticaleval}
\end{table}

\begin{table}[!h]
    \centering
    \caption{We repeat the same experiment as Tab.\ref{tab:theoreticaleval} with $s=20$ and $n=1k$ samples.
        }
    \resizebox{8.0cm}{!}{
    \begin{tabular}{c @{\hspace{2em}} c @{\hspace{0.1 em}} c @{\hspace{2em}} c @{\hspace{0.1em}} c}
        
        %GT & Mean $\hat{p}_0$ & Std $\hat{p}_0$ & Mean $\hat{p}_0$ &  Std $\hat{p}_0$ \\
      
        \toprule
        GT & \multicolumn{2}{c}{Sampled-based estimates} & \multicolumn{2}{c}{Model-based estimates}
        \\\cmidrule(lr){1-1} \cmidrule(lr){2-3} \cmidrule(lr){4-5} 
        &$\Ddot{\mu}_{\phat_0}$ & $\sqrt{\Ddot{\sigma}^2_{\phat_0}}$ & $\Tilde{\mu}_{\phat_0}$ &  $\sqrt{\Tilde{\sigma}^2_{\phat_0}}$ \\
        
        \midrule
        \multicolumn{5}{c}{Gender, $\balpha$=[0.976,0.979]}\\
        \midrule
        $p^*_0=0.9$ &0.855 & 0.0201 & 0.881  & 0.0106\\
        $p^*_0=0.8$ &0.774 & 0.0211 & 0.785  & 0.0135\\
        $p^*_0=0.7$ &0.672 & 0.0219 & 0.690  & 0.0152\\
        $p^*_0=0.6$ &0.580 & 0.0181 & 0.594  & 0.0162\\
        $p^*_0=0.5$ &0.510 & 0.0230 & 0.499  & 0.0164\\
        \midrule
        \multicolumn{5}{c}{$\balpha$=[0.881,0.887], Black-Hair}\\
        \midrule
        $p^*_0=0.9$ &0.768 & 0.180 & 0.804  &	0.0139\\
        $p^*_0=0.8$ &0.712 & 0.210 & 0.727  &	0.0162\\
        $p^*_0=0.7$ &0.658 & 0.190 & 0.650 &	0.0177\\
        $p^*_0=0.6$ &0.554 & 0.230 & 0.574   & 0.0186\\
        $p^*_0=0.5$ &0.508 & 0.242 & 0.497  &	0.0189
    \end{tabular}}
    \label{tab:theoreticalevals20n1k}
\end{table}
\begin{table}[!t]
    \centering
    \caption{We repeat the same experiment as Tab.\ref{tab:theoreticaleval} with $s=30$ and $n=500$ samples.
        }
    \resizebox{8.0cm}{!}{
    \begin{tabular}{c @{\hspace{2em}} c @{\hspace{0.1 em}} c @{\hspace{2em}} c @{\hspace{0.1em}} c}
        
        %GT & Mean $\hat{p}_0$ & Std $\hat{p}_0$ & Mean $\hat{p}_0$ &  Std $\hat{p}_0$ \\
      
        \toprule
        GT & \multicolumn{2}{c}{Sampled-based estimates} & \multicolumn{2}{c}{Model-based estimates}
        \\\cmidrule(lr){1-1} \cmidrule(lr){2-3} \cmidrule(lr){4-5} 
        &$\Ddot{\mu}_{\phat_0}$ & $\sqrt{\Ddot{\sigma}^2_{\phat_0}}$ & $\Tilde{\mu}_{\phat_0}$ &  $\sqrt{\Tilde{\sigma}^2_{\phat_0}}$ \\
        
        \midrule
        \multicolumn{5}{c}{Gender, $\balpha$=[0.976,0.979]}\\
        \midrule
        $p^*_0=0.9$ &0.860 & 0.0232 & 0.881  & 0.0149\\
        $p^*_0=0.8$ &0.780 & 0.0286 & 0.785  & 0.0191\\
        $p^*_0=0.7$ &0.710 & 0.0294 & 0.690  & 0.0215\\
        $p^*_0=0.6$ &0.578 & 0.0380 & 0.594  & 0.0228\\
        $p^*_0=0.5$ &0.520 & 0.0321 & 0.499  & 0.0233\\
        \midrule
        \multicolumn{5}{c}{$\balpha$=[0.881,0.887], Black-Hair}\\
        \midrule
        $p^*_0=0.9$ &0.742 & 0.0312 & 0.804  &	0.0197\\
        $p^*_0=0.8$ &0.740 & 0.0332 & 0.727  &	0.0229\\
        $p^*_0=0.7$ &0.610 & 0.0291 & 0.650  &	0.0250\\
        $p^*_0=0.6$ &0.582 & 0.350 & 0.574  & 0.0262\\
        $p^*_0=0.5$ &0.542 & 0.388 & 0.497  &	0.0267
    \end{tabular}}
    \label{tab:theoreticalevals30n500}
\end{table}

\FloatBarrier

\subsection{Goodness-Of-Fit Test: $\phat$ from the Real GAN in \cite{choiFairGenerativeModeling2020a} with Our Theoretical Model}
\begin{table}[!h]
    \centering
   \caption{\textbf{Validating theoretical model on GAN:} KS-test on $s=30$ and $\delta=0.05$ with $D_{crit}=0.24$. As seen from the table, since $\eta<D_{crit}$, all of the generated samples by GANs are statistically similar to the respective Gaussian at a 95\% confidence of the K-S test. }
   \resizebox{5cm}{!}{
    \begin{tabular}{c @{\hspace{1em}} c @{\hspace{1em}} c}
        Model Type & LA & $\eta$  \\
    \toprule
        Unweighted &  Gender & 0.1048 \\
        imp-weighted &  Gender & 0.1509 \\
        Unweighted &  Blackhair & 0.1065\\
        imp-weighted &  Blackhair & 0.1079
    \end{tabular}
    }
    \label{tab:KStest}
\end{table}
%Similar to \cref{sub:validatetheoreticalfakeG}, we would like to first evaluate if our Gaussian model is also a good representation for the $\phat$ samples from our GAN. 
%-------------Setup/objective that we agreed upon--------------------------
In order to make sure that our proposed theoretical model in Eqn. 3 and Eqn. 4 of the main paper, is also a good representation of $\phat$ when using a real GAN as generator, here we perform a goodness of fit test between proposed model for distribution of $\phat$, and sample data generated by a GAN.
%the empirical model estimated from the GAN samples.
To do this, we first obtain $s=30$ values of $\phat$ from framework shown in Fig. 2 of the main paper, when a respective StyleGANv2 from \cite{choiFairGenerativeModeling2020a} is used as generative model. 
%-------------Setup/objective that we agreed upon--------------------------
Recall that we showed in Sec. \ref{sec:sampleBasedEstimate} that the sample-based estimate is a good approximation of the theoretical model.
Hence, we use the sample-based estimates in Eqn. 5 and Eqn. 6 of the main paper to approximated mean and variances of the theoretical model's 
%\textcolor{red}{[Milad: Proposed model or Empirical model? Here we are using samples to estimate empirical model. Is that right?]}
Gaussian distribution, $\mathcal{N}(\Ddot{\mu}_{\phat_0},\Ddot{\sigma}^2_{\phat_0})$.

Now with both our model distribution and the GAN samples,
%sample-based empirical distribution, 
we utilise the Kolmogorov-Smirnov goodness of fit test (K-S test) to determine if the samples distribution is statistically similar to the proposed Gaussian model.
We thus propose the following hypothesis test for the samples $\phat^i_j, i \in \{1, \cdots, s\}$: 

\begin{flalign*}
&\mathbf{H_0}: \textit{the samples $\phat^i_j$
 belong to the modelled distribution.}&&\\
&\mathbf{H_1}: \textit{at least one of the samples $\phat^i_j$ does not match the modelled distribution.}&&
\end{flalign*}

The K-S test then measures a D-statistic ($\eta$) and compares it against a $D_{crit}$ for a given $s$. As we use $s=30$, and a significance level $\delta=0.05$ in our setup, we have $D_{crit}=0.24$. 
As seen from Tab. \ref{tab:KStest}, all of the measured $\eta$ values are below $D_{crit}$, 
thus we cannot reject the null hypothesis at a $95\%$ confidence with the K-S test. 
Therefore, we conclude that the distribution of the obtained samples from the framework (by GANs as generator) are statistically similar to the proposed Gaussian distribution. As a result, we can utilise CLEAM to approximate the $\pstar$ range in the presence of a real GAN as the generator.

%In Section 6.1 of the main paper, we discuss that samples of $\phat$ obtained from real GAN generators in \cite{choiFairGenerativeModeling2020a} follow a Gaussian distribution.
%Here, we 
We further perform a Quantile-Quantile(QQ) analysis to provide a more visual representation. In particular, we plot the Quantile-Quantile(QQ) plot between the $\phat$ samples (produced for the data generated by the GAN) and proposed model.
%man_24Nov: what are the parameters of this Gaussian model? how did you calculate?
As seen in Fig. \ref{fig:QQplot}, the  $\phat$ samples from GAN correlate tightly with the standardised line (in red), a line indicating a perfect correlation between theoretical and sample quantiles. This analysis supports our claim that the $\phat$ samples from a real generator (GAN) follow the distribution estimated by the proposed model.

%the  $\phat$ samples from the 
%real GAN generators in \cite{choiFairGenerativeModeling2020a} \textcolor{red}{(Can we say this a bit general? e.g.: 'the $\phat$ samples from a real generator (GAN) follow the distribution estimated by the proposed model.')} follow a Gaussian distribution.
\begin{figure*}[!h]
    \centering
    \begin{subfigure}[b]{0.5\textwidth}
        \centering
        \includegraphics[height=1.6in]{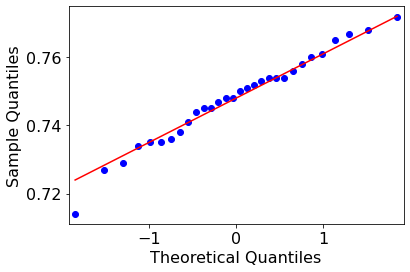}
        \caption{Unweighted, $\texttt{Gender}$.}
    \end{subfigure}%
    \begin{subfigure}[b]{0.5\textwidth}
        \centering
        \includegraphics[height=1.6in]{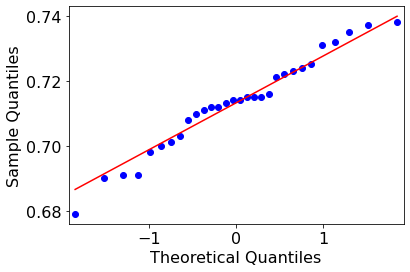}
        \caption{Weighted, $\texttt{Gender}$}
    \end{subfigure}%
    \newline
        \begin{subfigure}[b]{0.5\textwidth}
        \centering
        \includegraphics[height=1.6in]{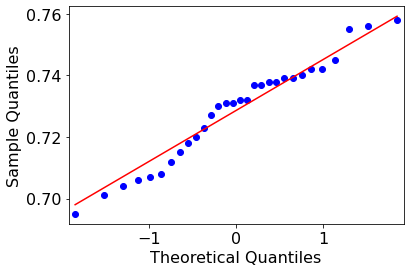}
        \caption{Unweighted, $\texttt{Blackhair}$}
    \end{subfigure}%
    \begin{subfigure}[b]{0.5\textwidth}
        \centering
        \includegraphics[height=1.6in]{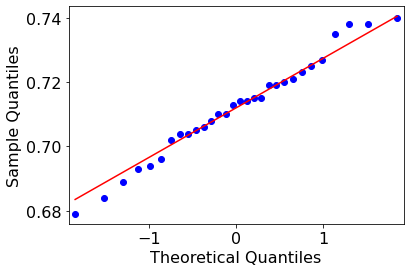}
        \caption{Weighted, $\texttt{BlackHair}$}
    \end{subfigure}%
     \caption{Quartile-Quartile(QQ) plot between $s=30$ $\phat$ samples calculated for StyleGANv2 \cite{karrasStyleBasedGeneratorArchitecture2019} generators and proposed theoretical model for $\phat$ (a Gaussian distribution in Eqn. 3, 4 of the main paper)}
    \label{fig:QQplot}
\end{figure*}

\section{Hyper-Parameter Settings in Our Experiments}

\paragraph{\bfseries\boldmath Attribute Classifier {$C_{u}$}.} 
In the majority of our experiments, unless stated otherwise, we utilised a ResNet-18 \cite{heDeepResidualLearning2016} classifier trained with an Adam optimiser\cite{kingmaAdamMethodStochastic2017} with a learning rate=$1e^{-3}$, Batch size=$64$ and input dim=$64$x$64$ from the CelebA dataset \cite{liuDeepLearningFace2015}. 

\paragraph{\bfseries\boldmath Generator $G_\phi$.}
As mentioned in the main paper, we utilised Choi \etal setup for the training of our imp-weighted \cite{choiFairGenerativeModeling2020a} and unweighted GANs. With this, we replicate their hyperparameter selection of $64$ x $64$ celebA \cite{liuDeepLearningFace2015} images with a learning rate=$2e^{-4}$, $\beta_1=0$, $\beta_2=0.99$ and four discriminator steps per generator step. We utilise a single 2080Ti for the training of our models.
For MaGNET \cite{humayunMaGNETUniformSampling2021a}, we utilised the saved model weights for a StyleGANv2 \cite{karrasStyleBasedGeneratorArchitecture2019} as well as, the pre-computed latent vectors $z$ and $MaGNET(z)$ provided by \cite{humayunMaGNETUniformSampling2021a} to generate the respective $s*n$ samples.  

\paragraph{\bfseries\boldmath Batch Size $s$.}
In our experiments, where we generated $n=1K$ samples with our pseudo-generator setup for $s$ batches, followed by applying CLEAM to approximate $\pstar$, we found that the batch size $s=30$ to be suitable to approximate the known GT $\pstar$.
Increasing $s$ did not lead to noticeable improvement in the error.
Following this, we utilised same parameters; $s=30$ and $n=1k$ samples generated from our trained GAN and approximate $\pstar$ with CLEAM, as per Table. 1 in the main paper. During which we computed the average time taken from the generation of $s=30$ and $n=1k$ samples over 5 runs for each of the 4 GANs, followed by the application of CLEAM, to be one minute and forty seconds.

\section{Additional Analysis}
\subsection{Retraining VGG-16 for Diversity\cite{keswaniAuditingDiversityUsing2021} Measures}
\label{sec:DiversitySetup}
In this section, we describe our experimental setup for Diversity \cite{keswaniAuditingDiversityUsing2021}, as utilised in Sec. 5 and 6 of the main paper.
Recall that in \cite{keswaniAuditingDiversityUsing2021} a VGG-16 \cite{simonyanVeryDeepConvolutional2014} model pre-trained on ImageNet \cite{dengImageNetLargescaleHierarchical2009} is utilised as a feature extractor. Then these features are fed into a similarity algorithm to measure Diversity.
From our initial results, on the pseudo-generator's setup in Fig. \ref{fig:VGG16imageNet} , we recognise that the original implementation with VGG-16 trained on ImageNet worked well on LA $\texttt{Gender}$. 
To demonstrate this, we compare our measured proxy diversity score against the GT diversity score shown in Eqn. \ref{eqn:GTDiversity}, as per \cite{keswaniAuditingDiversityUsing2021}.
\begin{equation}
    GT \, Diversity =\pstar_0 - \pstar_1
    \label{eqn:GTDiversity}
\end{equation}
However, when measuring harder LA $\texttt{BlackHair}$, we observed significant error between the GT Diversity scores and the proxy Diversity scores. 
This error was especially prevalent in the larger biases \eg $\pstar_0=0.9$. We theorised that, this was due to the differences between the domains \ie ImageNet versus CelebA.

To verify this, we retrained the VGG-16 model on the CelebA dataset with the respective LA. 
Then we removed the last fully connected layer of the classifier model, and utilise the 4096 feature vector for the diversity measurement, as per \cite{keswaniAuditingDiversityUsing2021}. From our results in Fig. \ref{fig:VGG16CelebA}, we see significant improvement in our implementation on both the LA $\texttt{Gender}$ and $\texttt{BlackHair}$. 

However, we recognise certain limitations in the Diversity measure when used on more ambiguous and harder LA $\texttt{Young}$ and $\texttt{Attractive}$. As per the previous LA, we first re-trained the VGG-16 model on the respective LA and measured their accuracies on a validation dataset. We noted an average accuracy of $78.44\%$ and $84.41\%$ for $\texttt{Young}$ and $\texttt{Attractive}$. Next, we removed the last layer of the classifier and utilised the 4096 feature vector for the implementation of diversity, as per \cite{keswaniAuditingDiversityUsing2021}. Unlike the original classifier (with the last fully connected layer) the same models were unable to accurately measure the respective $\pstar_0$ (biases) with the diversity algorithm, as seen in Fig. \ref{fig:VGG16AttractiveYoung}. From this, we observe that even our fined tuned VGG-16 feature extractor did not improve the Diversity framework on these harder LA.

%We conclude that the final fully connected layer is vital for the recognition of these harder LA. \textcolor{red}{(We don't need to include this as we don't have enough analysis. We may simply say that 'even fine-tuned version of Diversity is not working well for harder LAs'.)}

\begin{figure}[h!]
\begin{subfigure}[b]{\textwidth}
       \centering
    \includegraphics[width=\textwidth]{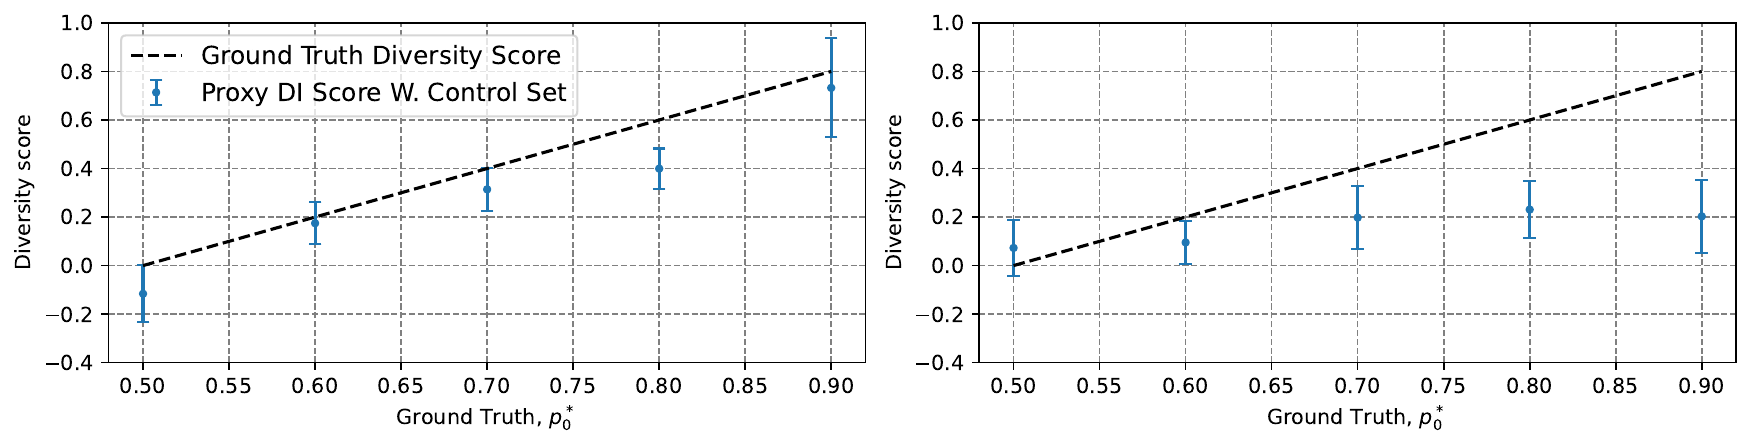}
    \caption{VGG-16 trained on ImageNet}
    \label{fig:VGG16imageNet} 
\end{subfigure}
\begin{subfigure}[b]{\textwidth}
       \centering
    \includegraphics[width=\textwidth]{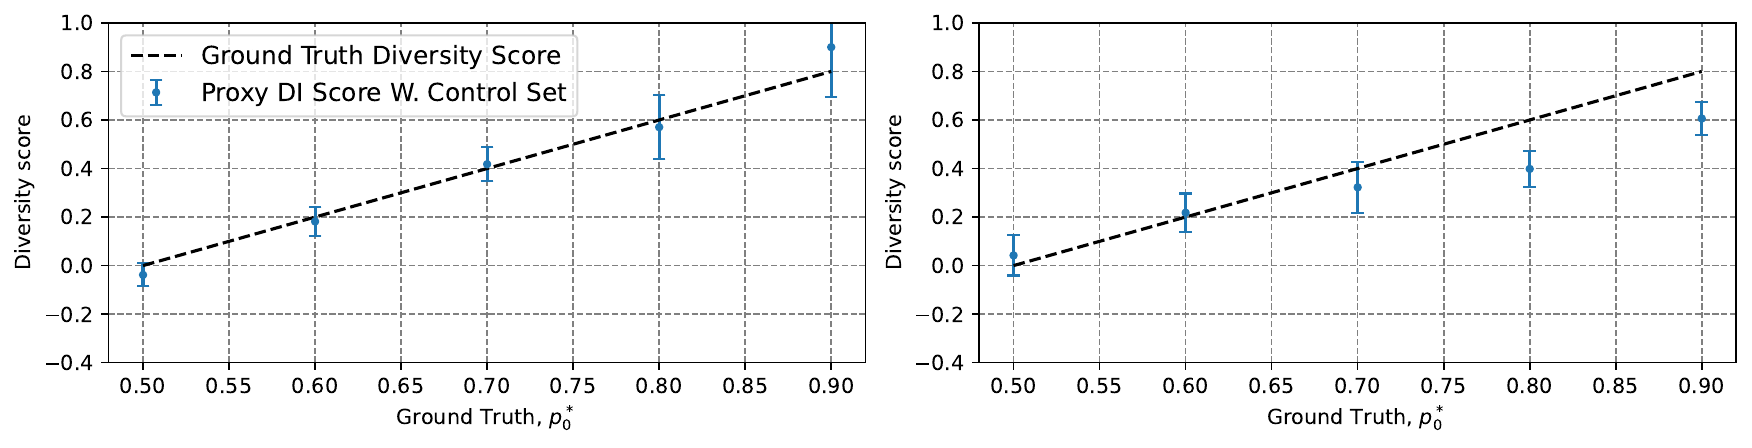}
    \caption{VGG-16 trained on CelebA}
    \label{fig:VGG16CelebA}  
\end{subfigure}
    \caption{{\bf Improvement in Diversity by fine-tuning the VGG-16, as a feature extractor}:
    %\textcolor{red}{(as feature extractor? if yes, please also include a brief description in paragraph 2 of D2)}:} 
    \textbf{(a)} Diversity implementation by \cite{keswaniAuditingDiversityUsing2021} with VGG-16 pre-trained on ImageNet as the feature extractor testing on the pseudo-generator's with $\pstar=\{0.9,0.8,0.7,0.6,0.5\}$ for LA $\texttt{Gender}$(Left) and $\texttt{BlackHair}$(Right).
    \textbf{(b)} We re-implemented VGG-16 and retrained with CelebA as the feature extractor. We observed significant improvement in predicting the GT $\pstar$}
\end{figure}
\begin{figure}[h!]
\begin{subfigure}[b]{0.5\textwidth}
       \centering
    \includegraphics[width=\textwidth]{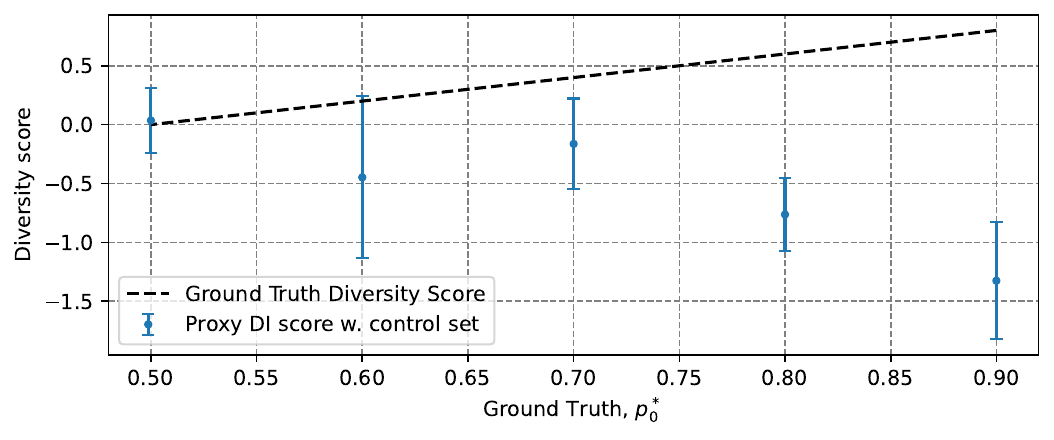}
    \caption{VGG-16(CelebA) on $\texttt{Attractive}$}
\end{subfigure}
\begin{subfigure}[b]{0.5\textwidth}
       \centering
    \includegraphics[width=\textwidth]{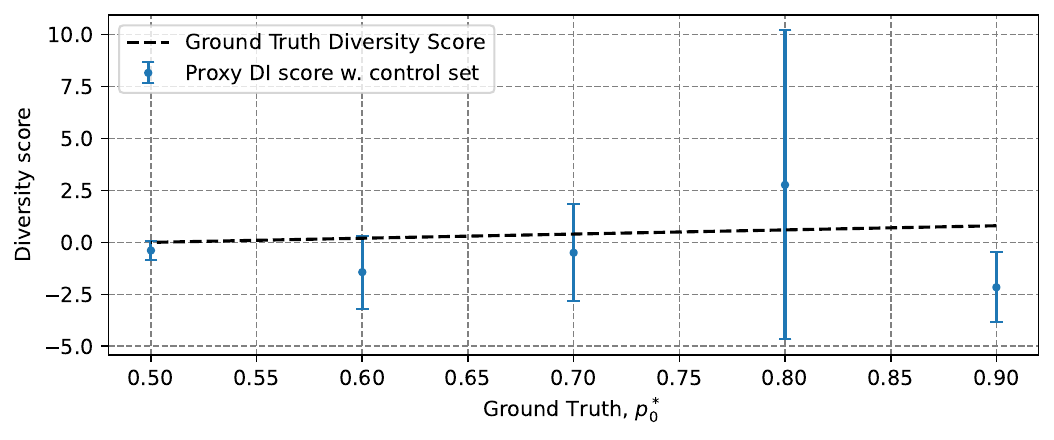}
    \caption{VGG-16(CelebA) on $\texttt{Young}$}
\end{subfigure}
    \caption{\textbf{Limitations Of Diversity
    algorithm.} %Implementation 
    %(\textcolor{red}{implementation or algorithm?})}.
    Our implementation of VGG-16 trained on CelebA on LA $\texttt{Attractive}$ and $\texttt{Young}$. VGG-16 Classifier achieved an accuracy of $78.44\%$ and $84.1\%$ for LA $\texttt{Attractive}$ and $\texttt{Young}$. However, the same VGG-16 performs poorly on the diversity metric, demonstrating the limitations of the diversity framework. }
    \label{fig:VGG16AttractiveYoung}
\end{figure}

\clearpage
\FloatBarrier
\subsection{Results of Proposed CLEAM on Different LA ($\texttt{Young}$, $\texttt{Attractive}$)}

In Sec. 5 of the main paper, we demonstrate CLEAM's ability to improve accuracy in approximating $\pstar$ with LA $\texttt{Gender}$ and $\texttt{BlackHair}$. In this section, we extend the experiment on harder (lower $\balpha$) LAs including $\texttt{Young}$, and $\texttt{Attractive}$. We further demonstrate that the Baseline is also sensitive to  $skew_\balpha=(\alpha_1-\alpha_0)$.

%In Section 5.2 of the main paper, we point out that the baseline method has a lower error at one specific test point, $\pstar=[0.5,0.5]$. However, we argue   that this should not be mistaken as better performance. We state that this observation is due to the specific combination of (i) Generator producing almost perfectly unbias data with $\pstar=[0.5,0.5]$ (ii) latent attribute classifier with almost perfectly  uniform inaccuracies $\balpha$. These lead to perfectly uniform misclassification, giving rise to the  false impression of better accuracy using the baseline method, at $\pstar=[0.5,0.5]$.  

\textbf{\em In this setup,} we repeat the same experiment with the pseudo-generator, but instead on LA $\texttt{Young}$ and $\texttt{Attractive}$ from the CelebA dataset. Given that both LA classifiers trained on either $\texttt{Young}$ or $\texttt{Attractive}$ have similar average accuracy, $\alpha_{Avg}=\frac{\alpha_0+\alpha_1}{2}$ of $0.801$ and $0.794$ but different $skew_\balpha$ of 0.103 and 0.027, we are able to investigate the effects of $skew_\balpha$ on both CLEAM and Baseline. We did not include Diversity in this study, due to its poor performance on harder LA, as discussed in \ref{sec:DiversitySetup}.
%in Tab. \ref{tab:peYoungAttractive}, \ref{tab:ieYoungAttractive}, who's $\balpha$ are skewed at different degrees, although having similar $\alpha_{Avg}=\frac{\alpha_0+\alpha_1}{2}$ of $0.801$ and $0.794$ respectively. The skew in $\balpha$ is defined as the difference between $\alpha_0$ and $\alpha_1$ \ie skew=$|\alpha_0-\alpha_1|$.

\textbf{\em From our results in Tab.\ref{fig:VGG16AttractiveYoung},}  we observe that as the $skew_\balpha$ increases from LA $\texttt{Attractive}$ to $\texttt{Young}$, the error becomes much more significant in the baseline method. The average Baseline $e_\mu$ increases from $12.3\%$ to $17.6\%$. On the other hand, CLEAM's $e_\mu$ remains below $1\%$, further emphasising CLEAM's effectiveness. Similar observation can be made for the interval estimates in Tab.\ref{tab:ieYoungAttractive}.

Furthermore, we observe that $skew_\balpha$ has influence on the errors observed in the lower biases \eg  $\pstar=[0.5,0.5]$. Unlike $\texttt{Gender}$ and $\texttt{Blackhair}$, who have relatively negligible skew, $\texttt{Young}$ and $\texttt{Attractive}$ observes a significantly larger error on $\pstar=[0.5,0.5]$. We attribute this 
%that LA with low $skew_\balpha$ observes lower error at $\pstar=[0.5,0.5]$ due 
to the specific combination of (i) Generator producing almost perfectly unbias data with $\pstar=[0.5,0.5]$ (ii) LA classifier with almost perfectly uniform inaccuracies $\balpha'=1-\balpha$ \ie $skew_\balpha \approx 0$. These lead to uniform misclassification, giving rise to the  false impression of better accuracy by the baseline method, at $\pstar=[0.5,0.5]$.  

\begin{table*}[!t]
    \centering
    \caption{Comparing \textbf{\em point estimate values} of 
    Baseline \cite{choiFairGenerativeModeling2020a},
    %, Diversity \cite{keswaniAuditingDiversityUsing2021} 
    and proposed CLEAM measurement framework on  (A) pseudo-generator with LA $\{\texttt{Young},\texttt{Attractive}\}$.}
\resizebox{7cm}{!}{
      \begin{tabular}{c  c @{\hspace{0.5em}} c @{\hspace{1em}} c @{\hspace{0.5em}} c @{\hspace{1em}} c @{\hspace{0.5em}} c}
        \toprule
        \multicolumn{7}{c}{\bf (A) Pseudo-Generator}\\
        \midrule
        \textbf{Test} & \multicolumn{2}{c}{\textbf{Baseline}\cite{choiFairGenerativeModeling2020a}}%& \multicolumn{2}{c}{\textbf{Diversity}\cite{keswaniAuditingDiversityUsing2021}}
        & \multicolumn{2}{c}{\textbf{(Ours) CLEAM}}
        \\
         \cmidrule(lr){1-1}\cmidrule(lr){2-3}\cmidrule(lr){4-5} \cmidrule(lr){6-7}
        %Baseline
        &$\mu_{\texttt{Base}}(\pstar_0)$ & $e_\mu(\pstar_0)$ 
         %Diversity
    %     &$\mu_{\texttt{Div}}(\pstar_0)$ & $e_\mu(\pstar_0)$ 
         %CLEAM
        &$\mu_{\texttt{CLEAM}}{\texttt(\pstar_0)}$ & $e_\mu(\pstar_0)$\\
        \midrule
        \multicolumn{7}{c}{$\balpha$=[0.749,0.852], \texttt{Young}}\\
        \midrule
         $p^*_0=0.9$ & 
        %Baseline
        0.690 & $23.3\%$  & 
        %Diversity
    %    - & - & 
        %CLEAM
        0.905& $\mathbf{0.5}\%$  
        \\  \hdashline
        $p^*_0=0.8$ & 
        %Baseline
        0.630 & $21.2\%$  &  
        %Diversity
    %    - & - & 
        %CLEAM
        0.804 & $\mathbf{0.5}\%$  
        \\ \hdashline
        $p^*_0=0.7$ & 
        %Baseline
        0.570 & $18.6\%$  & 
        %Diversity
    %    - & -  & 
        %CLEAM
        0.698& $\mathbf{0.2}\%$
        \\ \hdashline
        $p^*_0=0.6$ & 
        %Baseline
        0.510 & $15.0\%$  & 
        %Diversity
    %    - & -  & 
        %CLEAM
        0.595 & $\mathbf{0.8}\%$
        \\ \hdashline
        $p^*_0=0.5$ & 
        %Baseline
        0.450 & $10.0\%$  & 
        %Diversity
    %    - & - &
        %CLEAM
        0.506 & $\mathbf{1.2}\%$
        \\ \midrule
        &Avg Error& $17.6\%$ 
   %     &Avg Error&$-\%$ 
        &Avg Error&$\mathbf{0.64}\%$\\
        \midrule
        \multicolumn{7}{c}{$\balpha$=[0.780,0.807], \texttt{Attractive}}\\
        \midrule
        $p^*_0=0.9$ & 
        %Baseline
        0.730 & $18.8\%$  & 
        %Diversity
    %    - & -  & 
        %CLEAM
        0.908 & $\mathbf{0.9}\%$
        \\ \hdashline
        $p^*_0=0.8$ & 
        %Baseline
        0.670 & $16.3\%$  & 
        %Diversity
    %    - & -  & 
        %CLEAM
        0.804 & $\mathbf{0.5}\%$
        \\ \hdashline
        $p^*_0=0.7$ & 
        %Baseline
        $0.60$ & $14.3\%$  & 
        %Diversity
    %    - &  - & 
        %CLEAM
        0.696 & $\mathbf{0.6}\%$
        \\ \hdashline
        $p^*_0=0.6$ & 
        %Baseline
        0.54 & $10.0\%$ & 
        %Diversity
    %    - & -  & 
        %CLEAM
        $0.592$  & $\mathbf{1.3}\%$
        \\ \hdashline
        $p^*_0=0.5$ & 
        0.480 & $4.0\%$  & 
        %Diversity
    %    - & -  & 
        %CLEAM
        0.493 & $\mathbf{1.4}\%$  \\
        \hline 
        &Avg Error& $12.3\%$ 
    %    &Avg Error&$-\%$ 
        &Avg Error&$\mathbf{0.94}\%$\\
    \end{tabular}
    \label{tab:peYoungAttractive}
    }
\end{table*}

\begin{table*}[!t]
    \centering
    \caption{Comparing \textbf{\em interval estimate values} of 
    Baseline \cite{choiFairGenerativeModeling2020a}
    %, Diversity \cite{keswaniAuditingDiversityUsing2021} 
    and proposed CLEAM measurement framework on  (A) pseudo-generator with LA $\{\texttt{Young},\texttt{Attractive}\}$. 
    }
\resizebox{7cm}{!}{
      \begin{tabular}{c @{\hspace{1em}} c @{\hspace{0.5em}} c @{\hspace{1em}} c @{\hspace{0.5em}} c @{\hspace{1em}} c @{\hspace{0.5em}} c}
        \toprule
        \multicolumn{7}{c}{\bf (A) Pseudo-Generator}\\
        \midrule
        \textbf{Test} & \multicolumn{2}{c}{\textbf{Baseline}\cite{choiFairGenerativeModeling2020a}}& %\multicolumn{2}{c}{\textbf{Diversity}\cite{keswaniAuditingDiversityUsing2021}} & 
        \multicolumn{2}{c}{\textbf{(Ours) CLEAM}}
        \\
         \cmidrule(lr){1-1}\cmidrule(lr){2-3}\cmidrule(lr){4-5} \cmidrule(lr){6-7}
        %Baseline
        &$\rho_{\texttt{Base}}(\pstar_0)$ & $e_\rho(\pstar_0)$ 
         %Diversity
        % &$\rho_{\texttt{Div}}(\pstar_0)$ & $e_\rho(\pstar_0)$ 
         %CLEAM
        &$\rho_{\texttt{CLEAM}}{\texttt(\pstar_0)}$ & $e_\rho(\pstar_0)$\\
        \midrule
        \multicolumn{7}{c}{$\balpha$=[0.749,0.852], \texttt{Young}}\\
        \midrule
         $p^*_0=0.9$ & 
        %Baseline
        $[0.684,0.695]$ & $24.0\%$ & 
        %Diversity
       % - & -  & 
        %CLEAM
        $[0.890,0.920]$ & $\mathbf{2.2}\%$  
        \\  \hdashline
        $p^*_0=0.8$ & 
        %Baseline
        $[0.625,0.635]$ & $21.9\%$   & 
        %Diversity
      %  - &  - & 
        %CLEAM
        $[0.790,0.810]$ & $\mathbf{1.3}\%$  
        \\ \hdashline
        $p^*_0=0.7$ & 
        %Baseline
        $[0.565,0.575]$ & $19.2\%$ & 
        %Diversity
     %   - & -  & 
        %CLEAM
        $[0.690,0.710]$ & $\mathbf{1.4}\%$ 
        \\ \hdashline
        $p^*_0=0.6$ & 
        %Baseline
        $[0.505,0.515]$ &  $15.8\%$ & 
        %Diversity
     %   - & -  & 
        %CLEAM
        $[0.590,0.600] $ & $\mathbf{1.6}\%$ 
        \\ \hdashline
        $p^*_0=0.5$ & 
        %Baseline
        $[0.445,0.455]$ & $11.0\%$  & 
        %Diversity
    %    - & -  & 
        %CLEAM
        $[0.490,0.500]$ & $\mathbf{2.0}\%$
        \\ \midrule
        &Avg Error& $18.38\%$ 
   %     &Avg Error&$-\%$ 
        &Avg Error&$\mathbf{1.7}\%$\\
        \midrule
        \multicolumn{7}{c}{$\balpha$=[0.780,0.807], \texttt{Attractive}}\\
        \midrule
        $p^*_0=0.9$ & 
        %Baseline
        $[0.724,0.736]$ & $19.5\%$  & 
        %Diversity
    %    - & -  & 
        %CLEAM
        $[0.900,0.920]$ &  $\mathbf{2.2}\%$
        \\ \hdashline
        $p^*_0=0.8$ & 
        %Baseline
        $[0.665,0.675]$ & $16.9\%$ & 
        %Diversity
    %    - & -  &  
        %CLEAM
        $[0.790,0.810]$ & $\mathbf{1.3}\%$
        \\ \hdashline
        $p^*_0=0.7$ & 
        %Baseline
        $[0.594,0.606]$ & $15.1\%$ & 
        %Diversity
    %    - & -  & 
        %CLEAM
        $[0.690,0.710]$ & $\mathbf{1.4}\%$
        \\ \hdashline
        $p^*_0=0.6$ & 
        %Baseline
        $[0.534,0.546]$ & $11.0\%$ & 
        %Diversity
    %    - & -  & 
        %CLEAM
        $[0.580,0.600]$ & $\mathbf{3.3}\%$
        \\ \hdashline
        $p^*_0=0.5$ & 
        $[0.475,0.485]$ & $5.0\%$ & 
        %Diversity
    %    - & -  & 
        %CLEAM
        $[0.490,0.540]$ & $\mathbf{2.0}\%$  \\
        \hline 
        &Avg Error& $13.5\%$ &
    %    Avg Error&$-\%$ &
        Avg Error&$\mathbf{2.0}\%$\\
    \end{tabular}
    }
    \label{tab:ieYoungAttractive}
\end{table*}

\clearpage
\FloatBarrier
\subsection{Results of Proposed CLEAM with Different LA Classifiers (MobileNetV2\cite{sandlerMobileNetV2InvertedResiduals2018})}
In this section, we validate CLEAM's versatility with different classifier architecture. In our setup, we utilise MobileNetV2\cite{sandlerMobileNetV2InvertedResiduals2018} as in  \cite{frankelFairGenerationPrior2020}. We then measure the known GT $\pstar$ from the pseudo-generator with LA $\texttt{Gender}$ and $\texttt{BlackHair}$, as per Sec 5 of the main paper. Note that, as per MobileNetV2 architecture requirements, we resize the input images into $244$x$244$. 

As seen in our results in Tab. \ref{tab:MobileNetPE},\ref{tab:MobileNetIE}, MobileNetV2 demonstrates similar results, on the Baseline and CLEAM, to ResNet-18 model in the main paper. In these results, we observed a significantly large $e_\mu$ for the baseline of $1.4\%$ and $9.4\%$ for the LA $\texttt{Gender}$ and $\texttt{BlackHair}$. Whereas, CLEAM reported an $e_\mu$ of $0.8\%$ and $0.3\%$. The same can be observed in $e_\rho$. We thus demonstrates CLEAM's versatility and ability to be deployed as a post-processing method (without retraining), on models of varying architecture.

\begin{table*}[!h]
    \centering
    %New overall Caption
    \caption{Comparing \textbf{\em point estimate values} of Baseline \cite{choiFairGenerativeModeling2020a}, Diversity \cite{keswaniAuditingDiversityUsing2021} and proposed CLEAM measurement framework on (A) pseudo-generator with LA $\{\texttt{Gender},\texttt{BlackHair}\}$ and MobileNetV2\cite{sandlerMobileNetV2InvertedResiduals2018}.
    }
\resizebox{8.0cm}{!}{
      %\begin{tabular}{c  c @{\hspace{0.5em}} c @{\hspace{0.5em}} c @{\hspace{0.5em}} c @{\hspace{0.5em}} c @{\hspace{0.5em}} c @{\hspace{0.5em}} c @{\hspace{0.5em}} c @{\hspace{0.5em}} c @{\hspace{0.5em}} c@{\hspace{0.5em}}c @{\hspace{0.5em}} c}
      
      \begin{tabular}{c  c @{\hspace{0.5em}} c @{\hspace{1em}} c @{\hspace{0.5em}} c @{\hspace{1em}} c @{\hspace{0.5em}} c}
        \toprule
        \multicolumn{7}{c}{\bf (A) Pseudo-Generator}\\
        \midrule
        \textbf{Test} & \multicolumn{2}{c}{\textbf{Baseline}\cite{choiFairGenerativeModeling2020a}}& \multicolumn{2}{c}{\textbf{Diversity}\cite{keswaniAuditingDiversityUsing2021}} & \multicolumn{2}{c}{\textbf{(Ours) CLEAM}}
        \\
         \cmidrule(lr){1-1}\cmidrule(lr){2-3}\cmidrule(lr){4-5} \cmidrule(lr){6-7}
         %Baseline
        % &P.Est($p^*_0$) & Error &I.Est.($p^*_0$) & Max Error
        &$\mu_{\texttt{Base}}(\pstar_0)$ & $e_\mu(\pstar_0)$ 
         %Diversity
         %&P.Est.($p^*_0$) & Error &I.Est.($p^*_0$) & Max Error
         &$\mu_{\texttt{Div}}(\pstar_0)$ & $e_\mu(\pstar_0)$ 
         %CLEAM
        %& P.Est.($p^*_0$) & Error & I.Est.($p^*_0$) & Max Error
        &$\mu_{\texttt{CLEAM}}{\texttt(\pstar_0)}$ & $e_\mu(\pstar_0)$\\
        \midrule
        \multicolumn{7}{c}{$\balpha$=[0.980,0.986], \texttt{Gender}}\\
        \midrule
        $p^*_0=0.9$ & 
        %Baseline
        0.882 & 2.0  & 
        %Diversity
        $0.950$ & $5.6\%$ & 
        %CLEAM
        0.899 & $\mathbf{0.1}\%$
        \\ \hdashline
        $p^*_0=0.8$ & 
        %Baseline
         0.786 & $1.7\%$  & 
        %Diversity
        $0.785$ & $1.9\%$ &
        %CLEAM
         0.800 & $\mathbf{0.0}\%$
        \\ \hdashline
        $p^*_0=0.7$ & 
        %Baseline
        0.689 & $1.6\%$  & 
        %Diversity
        $0.709$ & $1.2\%$ & 
        %CLEAM
        0.699 & $\mathbf{0.1}\%$
        \\ \hdashline
        $p^*_0=0.6$ & 
        %Baseline
        0.593 & $1.2\%$  & 
        %Diversity
        $0.591$ & $1.5\%$ &
        %CLEAM
        0.600 & $\mathbf{0.0}\%$
        \\ \hdashline
        $p^*_0=0.5$ & 
        0.497 & $0.4\%$  & 
        %Diversity
        $0.481$ & $3.8\%$ & 
        %CLEAM
        0.502 & $\mathbf{0.3}\%$  \\
        \hline 
        &Avg Error& 1.4$\%$ &Avg Error&$2.8\%$ &Avg Error&$ \mathbf{0.8}\%$\\
        \midrule
        \multicolumn{7}{c}{$\balpha$=[0.861,0.916], \texttt{BlackHair}}\\
        \midrule
        $p^*_0=0.9$ & 
        %Baseline
        0.782 & $13.0\%$  & 
        %Diversity
        $0.803$ & $10.7\%$ & 
        %CLEAM
        0.899 & $\mathbf{0.1}\%$
        \\ \hdashline
        $p^*_0=0.8$ & 
        %Baseline
         0.705 & $11.8\%$  & 
        %Diversity
        $0.699$ & $12.6\%$ &
        %CLEAM
         0.800 & $\mathbf{0.0}\%$
        \\ \hdashline
        $p^*_0=0.7$ & 
        %Baseline
        0.623 & $10.3\%$  & 
        %Diversity
        $0.661$ & $5.5\%$ &
        %CLEAM
        0.700 & $\mathbf{0.0}\%$
        \\ \hdashline
        $p^*_0=0.6$ & 
        %Baseline
        0.550 & $8.3\%$  & 
        %Diversity
        $0.609$ & $1.5\%$ & 
        %CLEAM
        0.600 & $\mathbf{0.0}\%$
        \\ \hdashline
        $p^*_0=0.5$ & 
        0.478 & $3.8\%$  & 
        %Diversity
        $0.521$ & $4.2\%$ & 
        %CLEAM
        0.506 & $\mathbf{1.2}\%$  \\
        \hline 
        &Avg Error& $9.4\%$ &Avg Error&$6.9\%$ &Avg Error&$ \mathbf{0.3}\%$\\
        \bottomrule
    \end{tabular}
    }
    \label{tab:MobileNetPE}
\end{table*}

\newpage

\begin{table*}[!h]
    \centering
    %New overall Caption
    \caption{Comparing \textbf{\em Interval estimate values} of Baseline \cite{choiFairGenerativeModeling2020a}, Diversity \cite{keswaniAuditingDiversityUsing2021} and proposed CLEAM measurement framework on (A)
   % (\textcolor{red}{I think this (A) in all supp. tables have no use, and probably just remained because of Table 1 and 2 in the main paper.})
    pseudo-generator with LA $\{\texttt{Gender},\texttt{BlackHair}\}$ and MobileNetV2\cite{sandlerMobileNetV2InvertedResiduals2018}
    }
\resizebox{8.0cm}{!}{
      %\begin{tabular}{c  c @{\hspace{0.5em}} c @{\hspace{0.5em}} c @{\hspace{0.5em}} c @{\hspace{0.5em}} c @{\hspace{0.5em}} c @{\hspace{0.5em}} c @{\hspace{0.5em}} c @{\hspace{0.5em}} c @{\hspace{0.5em}} c@{\hspace{0.5em}}c @{\hspace{0.5em}} c}
      
      \begin{tabular}{c  c @{\hspace{0.5em}} c @{\hspace{1em}} c @{\hspace{0.5em}} c @{\hspace{1em}} c @{\hspace{0.5em}} c}
        \toprule
        \multicolumn{7}{c}{\bf (A) Pseudo-Generator}\\
        \midrule
        \textbf{Test} & \multicolumn{2}{c}{\textbf{Baseline}\cite{choiFairGenerativeModeling2020a}}& \multicolumn{2}{c}{\textbf{Diversity}\cite{keswaniAuditingDiversityUsing2021}} & \multicolumn{2}{c}{\textbf{(Ours) CLEAM}}
        \\
         \cmidrule(lr){1-1}\cmidrule(lr){2-3}\cmidrule(lr){4-5} \cmidrule(lr){6-7}
         %Baseline
        % &P.Est($p^*_0$) & Error &I.Est.($p^*_0$) & Max Error
        &$\rho_{\texttt{Base}}(\pstar_0)$ & $e_\rho(\pstar_0)$ 
         %Diversity
         %&P.Est.($p^*_0$) & Error &I.Est.($p^*_0$) & Max Error
         &$\rho_{\texttt{Div}}(\pstar_0)$ & $e_\rho(\pstar_0)$ 
         %CLEAM
        %& P.Est.($p^*_0$) & Error & I.Est.($p^*_0$) & Max Error
        &$\rho_{\texttt{CLEAM}}{\texttt(\pstar_0)}$ & $e_\rho(\pstar_0)$\\
        \midrule
        \multicolumn{7}{c}{$\balpha$=[0.980,0.986], \texttt{Gender}}\\
        \midrule
        $p^*_0=0.9$ & 
        %Baseline
        $[ 0.879 , 0.885 ]$ & $2.3\%$ & 
        %Diversity
        $[0.913 , 0.986 ]$ & $9.6\%$ &
        %CLEAM
        $[0.995,0.902]$ & $\mathbf{0.5}\%$  
        \\  \hdashline
        $p^*_0=0.8$ & 
        %Baseline
        $[ 0.782 , 0.790 ]$ & $2.3\%$ & 
        %Diversity
        $[0.762 , 0.809 ]$ & $4.8\%$ &
        %CLEAM
        $[0.794,0.804]$ & $\mathbf{0.6}\%$  
        \\ \hdashline
        $p^*_0=0.7$ & 
        %Baseline
        $[ 0.685, 0.693 ]$ & $2.1\%$ & 
        %Diversity
        $[0.696 , 0.722 ]$ & $3.1\%$ &
        %CLEAM
        $[0.694,0.704]$ & $\mathbf{0.8}\%$
        \\ \hdashline
        $p^*_0=0.6$ & 
        %Baseline
        $[ 0.585 , 0.597 ]$ & $2.5\%$  & 
        %Diversity
        $[0.581 , 0.612 ]$ & $3.3\%$ &
        %CLEAM
        $[594,0.605]$ & $\mathbf{1.0}\%$
        \\ \hdashline
        $p^*_0=0.5$ & 
        %Baseline
        $[ 0.491 , 0.502 ]$ & $1.8\%$  & 
        %Diversity
        $[0.473 , 0.490 ]$ & $5.5\%$ &
        %CLEAM
        $[495,0.507]$ & $\mathbf{1.1}\%$
        \\ \midrule
        &Avg Error& $2.2\%$ 
        &Avg Error&$5.3\%$ 
        &Avg Error&$\mathbf{0.8}\%$\\
        \midrule
        \multicolumn{7}{c}{$\balpha$=[0.861,0.916], \texttt{BlackHair}}\\
        \midrule
        $p^*_0=0.9$ & 
        %Baseline
        $[ 0.777 , 0.787 ]$ & $13.6\%$  & 
        %Diversity
        $[0.791 , 0.815 ]$ & $12.1\%$ &
        %CLEAM
        $[0.893,0.900]$ & $\mathbf{0.7}\%$
        \\ \hdashline
        $p^*_0=0.8$ & 
        %Baseline
        $[ 0.699 , 0.710 ]$ & $12.6\%$ & 
        %Diversity
        $[0.686 , 0.713 ]$ & $14.2\%$ &
        %CLEAM
        $[0.793,0.807]$ & $\mathbf{0.9}\%$
        \\ \hdashline
        $p^*_0=0.7$ & 
        %Baseline
        $[ 0.618 , 0.628 ]$ & $11.7\%$  & 
        %Diversity
        $[ 0.643 , 0.68 ]$ & $8.2\%$ &
        %CLEAM
        $[0.694,0.706]$ & $\mathbf{0.9}\%$
        \\ \hdashline
        $p^*_0=0.6$ & 
        %Baseline
        $[ 0.544 , 0.556 ]$ & $9.3\%$ & 
        %Diversity
        $[0.604 , 0.614 ]$ & $2.3\%$ &
        %CLEAM
        $[0.593,0.608]$ & $\mathbf{1.3}\%$
        \\ \hdashline
        $p^*_0=0.5$ & 
        $[ 0.472 , 0.484 ]$ & $5.6\%$ & 
        %Diversity
        $[0.506 , 0.536 ]$ & $7.2\%$ &
        %CLEAM
        $[0.498,0.514]$ & $\mathbf{2.4}\%$  \\
        \hline 
        &Avg Error& $10.6\%$ &Avg Error&$8.8\%$ &Avg Error&$\mathbf{1.2}\%$\\
        \bottomrule
    \end{tabular}}
    \label{tab:MobileNetIE}
\end{table*}
\newpage
\FloatBarrier
\subsection{Results of Proposed CLEAM with Different FD Measures}
Similarly, we demonstrate that CLEAM is effective in improving FD measures, regardless of the metric used. We used the results from Tab. \ref{tab:MobileNetPE} for this experiments. We then calculate $f$, the distance between a uniform distribution ($\bar{p}$) and the measured LA distribution ($\hat{p}$) \wrt the LA. Some examples of distance metrics used in previous works include, the L2-distance in \cite{choiFairGenerativeModeling2020a}, KL-divergence in \cite{tanImprovingFairnessDeep2020} and additionally L1-distance. 
We then compute the L1-error for the point estimate ($f_{est}$) against the GT $f$ ($f_{GT}$) of the  respective metric \ie $error=|f_{GT}-f_{est}|$. Note that $f_{est}$ is either the baseline or CLEAM point estimate of $f$. 
%Similarly, we calculate the max L1 distance for the interval estimates \ie $max\_error=max[|f_{GT}-f_{\mathcal{L}(\pstar)}|,|f_{GT}-f_{\mathcal{U}(\pstar)}|]$, where $f_{\mathcal{L}(\pstar)}$ and $f_{\mathcal{U}(\pstar)}$ are the lower and upper bound of the interval estimate of $f$. 
A lower error would indicate that the estimated $f$ is closer to the GT $f$ of its respective FD measure.

From Tab. \ref{tab:fakeG-FDm}, we observe that regardless of the $FD$ metric used, CLEAM produces the lowest error. Hence, we conclude that CLEAM can be utilised to improve FD measurements in fair generative models, independent on the metric used.
\begin{table*}[!h]
    \centering
    \caption{Based on the experiment in Tab. \ref{tab:MobileNetPE} we calculate $f$ with L1-distance, L2-distance and KL-divergence utilised in \cite{tanImprovingFairnessDeep2020,choiFairGenerativeModeling2020a,frankelFairGenerationPrior2020}. We then measured the L1 error \wrt GT $f$ for each of the point estimates. We observe that CLEAM is able to improve $f$ measurements \wrt the GT $f$, when compared against the baseline.}
\resizebox{6.1cm}{!}{
  %\begin{tabular}{|c|c|c|c|c||c|c|c|c|}
  \begin{tabular}{c cc @{\hspace{2em}} cc @{\hspace{2em}} ccccc}
        \toprule
        & \multicolumn{2}{c}{GT} & \multicolumn{2}{c}{Baseline} & 
        \multicolumn{4}{c}{(Ours) CLEAM}
        \\ \cmidrule(lr){2-3}\cmidrule(lr){4-5} \cmidrule(lr){6-9}
        &$p^*_0$ 
        & $f(\pstar)$ 
        & $f(\mu_{Base})$ 
        & Error
        & $f(\mu_{CLEAM})$ 
        & Error\\
         \midrule 
        \multicolumn{9}{c}{$\balpha$=[0.980,0.986], Gender}\\
        \midrule
        %\multicolumn{5}{|c|}{$\pstar=0.9$}\\
        KL & \multirow{3}{*}{$0.9$} & $0.531$ & $0.476$ & $0.052$ & $0.528$ & $\mathbf{0.003}$ \\
        L1 &                          & $0.8$   & $0.764$ & $0.034$ & $0.798$ & $\mathbf{0.002}$ \\
        L2 &                          & $0.566$   & $0.540$ & $0.024$ & $0.564$ & $\mathbf{0.002}$ \\
        \hline
        %\multicolumn{5}{|c|}{$\pstar=0.8$}\\
        KL & \multirow{3}{*}{$0.8$}  & $0.278$ & $0.251$ & $0.027$ & $0.277$ & $\mathbf{0.001}$\\
        L1 &                         & $0.6$   & $0.572$ & $0.028$ & $0.599$ & $\mathbf{0.001}$\\
        L2 &                         & $0.424$   & $0.405$ & $0.019$ & $0.424$ & $\mathbf{0.002}$\\
        \hline
        %\multicolumn{5}{|c|}{$\pstar=0.7$}\\
        KL & \multirow{3}{*}{$0.7$}  & $0.119$ & $0.106$ & $0.012$ & $0.118$ & $\mathbf{0.001}$ \\
        L1 &                         & $0.4$   & $0.378$ & $0.020$ & $0.398$ & $\mathbf{0.002}$ \\
        L2 &                         & $0.283$   & $0.267$ & $0.015$ & $0.282$ & $\mathbf{0.001}$ \\
        \hline
        %\multicolumn{5}{|c|}{$\pstar=0.6$}\\
        KL & \multirow{3}{*}{$0.6$}  & $0.0290$ & $0.0249$ & $0.0041$ & $0.0289$ & $\mathbf{1e^{-4}}$ \\
        L1 &                         & $0.2$    & $0.185$ & $0.015$ & $0.200$ & $\mathbf{0.0}$ \\
        L2 &                         & $0.141$   & $0.131$ & $0.010$  & $0.141$ & $\mathbf{0.0}$ \\
        \hline
        %\multicolumn{5}{|c|}{$\pstar=0.5$}\\
        KL & \multirow{3}{*}{$0.5$}  & $0.0$  & $1.95e^{-5}$ & $1.95e^{-5}$ & $1.01e^{-5}$ & $\mathbf{1.01e^{-5}}$  \\
        L1 &                         & $0.0$ & $5.2e^{-3}$ & $5.2e^{-3}$ & $3.8e^{-3}$ & $\mathbf{3.8e^{-3}}$ \\
        L2 &                         & $0.0$   & $3.68e^{-3}$ & $3.68e^{-3}$ & $2.65e^{-3}$ & $\mathbf{2.65e^{-3}}$ \\
        \hline 
        \multicolumn{9}{c}{$\balpha$=[0.861,0.916], Black Hair}\\
        \hline
        %\multicolumn{5}{|c|}{$\pstar=0.9$}\\
        KL & \multirow{3}{*}{$0.9$}  & $0.531$ & $0.244$ & $0.287$ & $0.530$ & $\mathbf{0.001}$  \\
        L1 &                         & $0.8$   & $0.565$ & $0.235$ & $0.799$ & $\mathbf{0.001}$  \\
        L2 &                          & $0.566$   & $0.399$ & $0.167$ & $0.565$ & $\mathbf{0.001}$  \\
        \hline
        %\multicolumn{5}{|c|}{$\pstar=0.8$}\\
        KL & \multirow{3}{*}{$0.8$} & $0.278$ & $0.125$ & $0.153$ & $0.278$ & $\mathbf{0.0}$ \\
        L1 &                        & $0.6$   & $0.410$ & $0.190$ & $0.600$ & $\mathbf{0.0}$ \\
        L2 &                          & $0.424$   & $0.290$ & $0.134$ & $0.424$ & $\mathbf{0.0}$ \\
        \hline
        %\multicolumn{5}{|c|}{$\pstar=0.7$}\\
        KL & \multirow{3}{*}{$0.7$} & $0.119$ & $0.0475$ & $0.0715$ & $0.118$ & $\mathbf{0.001}$ \\
        L1 &                        & $0.4$   & $0.255$ & $0.175$ & $0.400$ & $\mathbf{0.0}$ \\
        L2 &                          & $0.283$   & $0.180$ & $0.103$ & $0.283$ & $\mathbf{0.0}$ \\
        \hline
        %\multicolumn{5}{|c|}{$\pstar=0.6$}\\
        KL & \multirow{3}{*}{$0.6$} & $0.0290$ & $7.3e^{-3}$ & $0.0217$ & $0.0293$ & $\mathbf{3e^{-4}}$ \\
        L1 &                        & $0.2$    & $0.101$ & $0.099$ & $0.201$ & $\mathbf{0.001}$ \\
        L2 &                          & $0.141$   & $0.0712$ & $0.0698$ & $0.142$ & $\mathbf{0.001}$ \\
        \hline
        %\multicolumn{5}{|c|}{$\pstar=0.5$}\\
        KL & \multirow{3}{*}{$0.5$} & $0.0$ & $1.5e^{-3}$ & $1.5e^{-3}$ & $1.0e^{-4}$ & $\mathbf{1.0e^{-4}}$ \\
        L1 &                        & $0.0$ & $0.0452$ & $0.0452$ & $0.0123$ & $\mathbf{0.0123}$  \\
        L2 &                          & $0.0$  & $0.0320$ & $0.0320$  & $8.7e^{-3}$ & $\mathbf{8.7e^{-3}}$ \\
        \hline

    \end{tabular}
    }
    \label{tab:fakeG-FDm}
\end{table*}
\FloatBarrier
\iffalse
We recognise that our solution is dependent on the generator having a Gaussian distribution. Utilising the real GAN models in Sec. \ref{sub:exprealgan}, we generated $s=30$ samples of $n=1k$ and utilised a D’Agostino and Pearson’s $K^2$ test (DP-test) to compare these samples against a Gaussian. The DP-test utilises the skew and kurtosis of the sample data to make this statistical inference and outputs a p-vale. If the p-value were larger than the chosen $\delta$, then we have a confidence of $(1-\delta)*100\%$ that we cannot reject the null hypothesis that the sample distribution is Gaussian. As seen in Tab. \ref{tab:DAK2test}, all of our generators out $p-values>0.05$, giving us a $95\%$ confidence \wrt the DP-test that the samples are gaussian. 
\begin{table}[!h]
    \centering
    \begin{tabular}{c|c|c}
        Model Type & LA & P-value  \\
    \hline \hline
        Unweighted &  Gender & 0.528 \\
        imp-weighted &  Gender & 0.745 \\
        Unweighted &  Blackhair & 0.537\\
        imp-weighted &  Blackhair &  0.945
    \end{tabular}
    \caption{D’Agostino’s $K^2$ Test results}
    \label{tab:DAK2test}
\end{table}
\fi

\clearpage
\FloatBarrier
\subsection{Analysing CLEAM on MaGNET\cite{humayunMaGNETUniformSampling2021a}}
In this section, we provide the graphical illustration of Sec 6.2 of the main paper. 
%(\textcolor{red}{Are we reporting this because we just have it?}) \textcolor{blue}{We report this because we mentioned, "See supplementary for graphical illustration" in the main text, line 605}
\begin{figure}[!h]
    \begin{subfigure}{0.5\textwidth}
     \centering
    \includegraphics[scale=0.15]{FiguresAppendix/MaGNET/Gender_phat_plot_v2.pdf}
    \caption{LA, $\texttt{Gender}$}
    \end{subfigure}
    \begin{subfigure}{0.5\textwidth}
     \centering
    \includegraphics[scale=0.15]{FiguresAppendix/MaGNET/Blackhair_phat_plot_v2.pdf}
    \caption{LA, $\texttt{BlackHair}$}
    \end{subfigure}
    \caption{\textbf{Fair Generation with MaGNET\cite{humayunMaGNETUniformSampling2021a} Sampling:} Figures in the first and second rows are bias measurements of StyleGANv2\cite{karrasStyleBasedGeneratorArchitecture2019} with and without MaGNET\cite{humayunMaGNETUniformSampling2021a} sampling. In all figures, the Baseline and CLEAM PE/IE are included, i.e.,  $\mu_\ddagger(\pstar_0)$ and $\rho_\ddagger(\pstar_0)$ for $\ddagger\in \{\texttt{CLEAM},\texttt{Base}\}$.
    Taking accuracy of LA classifier into account, 
    CLEAM estimates (green) are rather different from the Baseline estimates (blue). This is especially noticeable for LA $\texttt{BlackHair}$ (b), when accuracy of LA classifier is lower.}
    \label{Fig:MaGNET}
\end{figure}

\FloatBarrier
\clearpage
\section{Interval Estimate}
\begin{table*}[!t]
    \centering
    %New overall Caption
    \caption{
    Comparing {\bf interval values} of Baseline \cite{choiFairGenerativeModeling2020a}, Diversity \cite{keswaniAuditingDiversityUsing2021} and our proposed CLEAM measurement framework in evaluating the $p^*$ of datasets sampled from (A) StyleGAN2 \cite{karrasStyleBasedGeneratorArchitecture2019} and (B) StyleSwim \cite{zhang2021styleswin}. 
    We utilize four different classifier Resnet-18/34 \cite{heDeepResidualLearning2016}, MobileNetv2 \cite{sandlerMobileNetV2InvertedResiduals2018} and VGG-16 \cite{simonyanVeryDeepConvolutional2014} to classify the SA, \texttt{Gender} and \texttt{Blackhair}, and measure their distribution.
    We then compared the measured values against the GT $p^*$ of the datasets and reported the mean errors with Eqn. \ref{eqn:intervalError}.}
\resizebox{14.0cm}{!}{
      \begin{tabular}{c c c @{\hspace{0.5em}} c @{\hspace{1em}} c @{\hspace{0.5em}} c @{\hspace{1em}} c @{\hspace{0.5em}} c}
        \toprule
        \multicolumn{8}{c}{\bf (A) StyleGAN2}\\
        \midrule
          \textbf{Classifier} &
          \textbf{GT} & \multicolumn{2}{c}{\textbf{Baseline}\cite{choiFairGenerativeModeling2020a}}& \multicolumn{2}{c}{\textbf{Diversity}\cite{keswaniAuditingDiversityUsing2021}} & \multicolumn{2}{c}{\textbf{(Ours) CLEAM}}
        \\
         \cmidrule(lr){1-1}\cmidrule(lr){2-2}\cmidrule(lr){3-4}\cmidrule(lr){5-6} \cmidrule(lr){7-8}
         %Baseline
        & &
        $\rho_{\texttt{Base}}(\pstar_0)$ & $e_\rho(\pstar_0)(\downarrow)$ 
         %Diversity
         &$\rho_{\texttt{Div}}(\pstar_0)$ & $e_\rho(\pstar_0)(\downarrow)$ 
         %CLEAM
        &$\rho_{\texttt{CLEAM}}{\texttt(\pstar_0)}$ & $e_\rho(\pstar_0)(\downarrow)$\\
        \midrule
        \multicolumn{8}{c}{\texttt{Gender}}\\
        \midrule
        ResNet-18 & \multirow{ 3}{*}{$p^*_0=0.642$}& 
        [$0.602$, $0.618$] & $6.1\%$ & 
        %Diversity
        $-.-$ & $-.-\%$ & 
        %CLEAM
       [$0.629$, $0.646$] & $\mathbf{1.9\%}$
        \\  \hdashline
        ResNet-34 & & 
        [$0.589$, $0.599$] & $8.1\%$ &
        %Diversity
        $-.-$ & $-.-\%$ &
        %CLEAM
        [$0.628$, $0.638$] & $\mathbf{2.2\%}$ 
        \\ \hdashline
        MobileNetv2 & & 
        [$0.602$, $0.612$] & $6.2\%$ &
        %Diversity
        $-.-$ & $-.-\%$ & 
        %CLEAM
        [$0.632$, $0.643$] & $\mathbf{1.6\%}$
        \\ \hdashline
        VGG-16 & & 
        [$0.526$, $0.538$] & $18.0\%$ &
        %Diversity
        $[0.536$ , $0.564]$ & $16.5\%$ & 
        %CLEAM
        [$0.628$, $0.644$] & $\mathbf{2.2\%}$
        \\ \hdashline
        \midrule
        & & Avg Error& $9.6\%$ 
        &Avg Error&$16.5\%$ 
        &Avg Error&$\mathbf{2.0}\%$\\
        \midrule
    %Blackhair
        \midrule
        \multicolumn{8}{c}{\texttt{Blackhair}}\\
        \midrule
        ResNet-18 & \multirow{ 3}{*}{$p^*_0=0.643$}& 
        [$0.591$, $0.607$] & $8.0\%$ & 
        %Diversity
        $-.-$ & $-.-\%$ & 
        %CLEAM
        [$0.631$, $0.652$] & $\mathbf{2.1\%}$
        \\  \hdashline
        ResNet-34 & & 
        [$0.561$, $0.572$] & $12.7\%$ &
        %Diversity
        $-.-$ & $-.-\%$ &
        %CLEAM
        [$0.637$, $0.651$] & $\mathbf{1.4\%}$ 
        \\ \hdashline
        MobileNetv2 & & 
        [$0.574$, $0.584$] & $10.7\%$ &
        %Diversity
        $-.-$ & $-.-\%$ & 
        %CLEAM
        [$0.632$, $0.647$] & $\mathbf{1.7\%}$
        \\ \hdashline
        VGG-16 & & 
        [$0.597$, $0.608$] & $5.9\%$ &
        %Diversity
        [$0.568$, $0.596$] & $11.7\%$ &
        %CLEAM
        [$0.632$, $0.648$] & $\mathbf{1.9\%}$\\
        \midrule
        & & Avg Error& $9.3\%$ 
        &Avg Error&$11.7\%$ 
        &Avg Error&$\mathbf{1.8}\%$\\
        \midrule
        \midrule
        \multicolumn{8}{c}{\bf (B) StyleSwin}\\
        \midrule
        %  \textbf{Classifier} &
        %%  \textbf{Test} & \multicolumn{2}{c}{\textbf{Baseline}\cite{choiFairGenerativeModeling2020a}}& \multicolumn{2}{c}{\textbf{Diversity}\cite{keswaniAuditingDiversityUsing2021}} & \multicolumn{2}{c}{\textbf{(Ours) CLEAM}}
        %\\
        % \cmidrule(lr){1-1}\cmidrule(lr){2-2}\cmidrule(lr){3-4}\cmidrule(lr){5-6} \cmidrule(lr){7-8}
         %Baseline
        %& &
        %$\mu_{\texttt{Base}}(\pstar_0)$ & $e_\mu(\pstar_0)$ 
         %Diversity
        % &$\mu_{\texttt{Div}}(\pstar_0)$ & $e_\mu(\pstar_0)$ 
         %CLEAM
        %&$\mu_{\texttt{CLEAM}}{\texttt(\pstar_0)}$ & $e_\mu(\pstar_0)$\\
        %\midrule
        \multicolumn{8}{c}{\texttt{Gender}}\\
        \midrule
        ResNet-18 & \multirow{ 3}{*}{$p^*_0=0.656$}& 
        [$0.612,0.629$] & $6.9\%$ & 
        %Diversity
        $-.-$ & $-.-\%$ & 
        %CLEAM
        [$0.639,0.658$] & $\mathbf{2.7\%}$ 
        \\  \hdashline
        ResNet-34 & & 
        [$0.605,0.615$] & $8.0\%$&
        %Diversity
        $-.-$ & $-.-\%$ &
        %CLEAM
        [$0.643,0.654$] & 
        $\mathbf{2.0}\%$  
        \\ \hdashline
        MobileNetv2 & & 
        [$0.618,0.629$] & $5.9\%$ & 
        %Diversity
        $-.-$ & $-.-\%$ & 
        %CLEAM
        [$0.649,0.661$]  & $\mathbf{1.3}\%$ 
        \\ \hdashline
        VGG-16 & & 
        [$0.549,0.560$] & $16.3\%$ & 
        %Diversity
        [$0.548,0.576$] & $16.4\%$ & 
        %CLEAM
        [$0.660,0.675$]  & $\mathbf{2.7}\%$ 
        \\
        \midrule
        & & Avg Error& $9.3\%$ 
        &Avg Error&$16.4\%$ 
        &Avg Error&$\mathbf{2.2}\%$\\
        \midrule
    %Blackhair
        \midrule
        \multicolumn{8}{c}{\texttt{Blackhair}}\\
        \midrule
        ResNet-18 & \multirow{ 3}{*}{$p^*_0=0.668$}& 
        [$0.605,0.620$] & $9.5\%$ &
        %Diversity
        $-.-$ & $-.-\%$ & 
        %CLEAM
        [$0.649,0.670$] & $\mathbf{2.9\%}$ 
        \\  \hdashline
        ResNet-34 & & 
        [$0.576,0.586$] & $11.8\%$&
        %Diversity
        $-.-$ & $-.-\%$ &
        %CLEAM
        [$0.656,0.669$] & 
        $\mathbf{1.9}\%$  
        \\ \hdashline
        MobileNetv2 & & 
        [$0.591,0.600$] & $12.7\%$ & 
        %Diversity
        $-.-$ & $-.-\%$ & 
        %CLEAM
        [$0.652,0.666$]  & $\mathbf{2.4}\%$ 
        \\ \hdashline
        VGG-16 & & 
        [$0.620,630$] & $7.7\%$ & 
        %Diversity
        [$0.590,0.626$] & $11.7\%$ & 
        %CLEAM
        [$0.670,0.684$]  & $\mathbf{2.4}\%$ 
        \\
        \midrule
        & & Avg Error& $10.4\%$ 
        &Avg Error&$11.7\%$ 
        &Avg Error&$\mathbf{2.4}\%$\\
        \midrule
    \end{tabular}
0    }
    \label{tab:G_IE}
\end{table*}
\begin{table*}[!t]
    \centering
    \caption{
    %{\color{red} To update.}
    Comparing \textbf{\em interval estimate values} of 
    Baseline \cite{choiFairGenerativeModeling2020a}, Diversity \cite{keswaniAuditingDiversityUsing2021} and proposed CLEAM measurement framework on both  (A) pseudo-generator and (B,C) real GANs with LA  \{\texttt{Gender}, \texttt{BlackHair}\}.
    To calculate IE, we use 95\% CI for Baseline, the converted 95\% CI for Diversity and Eqn. \ref{eqn:CIpstar} for proposed CLEAM. Similar to Tab. \ref{tab:fakeG_PE}, since for pseudo-generator the $\pstar$ is known, we report the interval max error $e_\rho$ using Eqn. \ref{eqn:intervalError}.
    For real GANs, we apply CLEAM to obtain more accurate IE for the fairness of GANs in  \cite{choiFairGenerativeModeling2020a,humayunMaGNETUniformSampling2021a}.}
\resizebox{14cm}{!}{
      \begin{tabular}{c  c @{\hspace{0.5em}} c @{\hspace{1em}} c @{\hspace{0.5em}} c @{\hspace{1em}} c @{\hspace{0.5em}} c}
        \toprule
        \multicolumn{7}{c}{\bf (A) Pseudo-Generator}\\
        \midrule
        \textbf{GT} & \multicolumn{2}{c}{\textbf{Baseline}\cite{choiFairGenerativeModeling2020a}}& \multicolumn{2}{c}{\textbf{Diversity}\cite{keswaniAuditingDiversityUsing2021}} & \multicolumn{2}{c}{\textbf{(Ours) CLEAM}}
        \\
         \cmidrule(lr){1-1}\cmidrule(lr){2-3}\cmidrule(lr){4-5} \cmidrule(lr){6-7}
        %Baseline
        % &P.Est($p^*_0$) & Error &I.Est.($p^*_0$) & Max Error
        &$\rho_{\texttt{Base}}(\pstar_0)$ & $e_\rho(\pstar_0)(\downarrow)$ 
         %Diversity
         %&P.Est.($p^*_0$) & Error &I.Est.($p^*_0$) & Max Error
         &$\rho_{\texttt{Div}}(\pstar_0)$ & $e_\rho(\pstar_0)(\downarrow)$ 
         %CLEAM
        %& P.Est.($p^*_0$) & Error & I.Est.($p^*_0$) & Max Error
        &$\rho_{\texttt{CLEAM}}{\texttt(\pstar_0)}$ & $e_\rho(\pstar_0)(\downarrow)$\\
        \midrule
        \multicolumn{7}{c}{$\balpha$=[0.976,0.979], \texttt{Gender}}\\
        \midrule
        $p^*_0=0.9$ & 
        $[0.876 , 0.884 ]$ & $2.7\%$ &
        %Diversity
        $[0.913 , 0.986 ]$ & $9.6\%$ &
        %CLEAM
        [$0.895$, $0.904$] & $\mathbf{0.5}\%$ 
        \\  \hdashline
        $p^*_0=0.8$ & 
        $[ 0.778   , 0.788  ]$ & $2.8\%$ 
        %Diversity
        & $[0.762 , 0.809 ]$ & $4.8\%$
        %CLEAM
        & [$0.794$, $0.803$] & $\mathbf{0.8}\%$
        \\ \hdashline
        $p^*_0=0.7$ & 
        $[ 0.687  , 0.695  ]$ & $1.9\%$ &
        %Diversity
        $[0.696 , 0.722 ]$ & $3.1\%$ &
        %CLEAM
        [$0.697$, $0.707$]  & $\mathbf{0.1}\%$
        \\ \hdashline
        $p^*_0=0.6$ & 
        $[0.586  , 0.598 ]$ & $2.3\%$&
        %Diversity
        $[0.581 , 0.612 ]$ & $3.3\%$ &
        %CLEAM
        [$0.591$,$0.603$]   & $\mathbf{1.5}\%$ 
        \\ \hdashline
        $p^*_0=0.5$ & 
        $[0.495  , 0.507 ]$ & $\mathbf{1.0}\%$ &
        %Diversity
        $[0.473 , 0.490 ]$ & $5.5\%$ &
        %CLEAM
        [$0.497$, $0.508$]  & $1.6\%$ \\
        \midrule
        & Avg Error & $2.1\%$ 
        &Avg Error& $5.26\%$
        &Avg Error& $\mathbf{0.90}\%$ \\
        \midrule
        \multicolumn{7}{c}{$\balpha$=[0.881,0.887], \texttt{BlackHair}}\\
        \midrule
        $p^*_0=0.9$ & 
        [$ 0.800  , 0.806 $] & $11.0\%$ &
        %Diversity
        $[0.791 , 0.815 ]$ & $12.1\%$ &
        %CLEAM
       [$0.893$, $0.905$] & $\mathbf{0.8}\%$ 
        \\ \hdashline
        $p^*_0=0.8$ & 
        [$0.719  , 0.727 $] & $10.1\%$ &
        %Diversity
        $[0.686 , 0.713 ]$ & $14.2\%$ &
        %CLEAM
        [$0.790$, $0.803$] & $\mathbf{1.3}\%$
        \\ \hdashline
        $p^*_0=0.7$ & 
        [$ 0.648  , 0.660  $] & $7.4\%$  &
        %Diversity
        $[ 0.643 , 0.68 ]$ & $8.2\%$ &
        %CLEAM
        [$0.698$, $0.712$]  & $\mathbf{1.6}\%$
        \\ \hdashline
        $p^*_0=0.6$ & 
        [$ 0.564  , 0.586  $] & $5.8\%$ &
        %Diversity
        $[0.604 , 0.614 ]$ & $2.3\%$ &
        %CLEAM
        [$0.599$, $0.606$]   & $\mathbf{1.0}\%$ 
        \\ \hdashline
        $p^*_0=0.5$ & 
        [$ 0.495  , 0.505  $] & $\mathbf{1.0}\%$ &
        %Diversity
        $[0.506 , 0.536 ]$ & $7.2\%$ &
        %CLEAM
        [$0.497$, $0.511$]  & $1.9\%$ \\
        \hline 
        & Avg Error&$7.06\%$ 
        &Avg Error& $8.8\%$
        &Avg Error& $\mathbf{1.32}\%$ \\
        \iffalse
        \toprule
        \multicolumn{7}{c}{\bf (B)   Importance Re-weighting \cite{choiFairGenerativeModeling2020a} GAN}\\
        \toprule
        \multicolumn{7}{c}{$\balpha$=[0.976,0.979], \texttt{Gender}}\\
        \midrule
        Unweighted & [$0.721  ,0.732 $] & - & [$0.711,0.736$] & - & [$0.733 ,0.744 $] & -  
        \\
        Weighted & [$0.705 ,0.716 $] & -  & [$0.697,0.723$] & - & [$0.716 ,0.728 $] & -\\
        \midrule
        \multicolumn{7}{c}{$\balpha$=[0.881,0.887], \texttt{BlackHair}}\\
         \midrule
        Unweighted & [$0.725 ,0.733 $] & - & [$0.718,0.743$] & -  & [$0.798 ,0.809 $] & -\\
        Weighted & [$0.710 ,0.722 $] & - & [$0.710,0.730$] & - & [$0.778 ,0.792 $] & -\\
        \toprule
        \multicolumn{7}{c}{\bf (C)  MaGNET Sampling \cite{humayunMaGNETUniformSampling2021a} GAN}\\
        \toprule
        \multicolumn{7}{c}{$\balpha$=[0.976,0.979], \texttt{Gender}}\\
        \midrule
        $z$ & [$ 0.562 , 0.570 $] & - & [$0.555,0.575$] & - & [ $0.566 , 0.574$ ] & - \\
        $MaGNET(z)$  & [$0.516 , 0.525$] & - & [$0.515,0.535$] & - & [$0.519 , 0.528$ ] & - \\    
        \midrule
        \multicolumn{7}{c}{$\balpha$=[0.881,0.887], \texttt{BlackHair}}\\
        \midrule
        $z$ & [ $0.543 , 0.552$ ] & -  & [$0.540,0.560$] & - & $[ 0.560 , 0.572$ ] & -  \\
        $MaGNET(z)$ & [ $0.568 , 0.577$ ] & - &  [$0.560,0.590$] & - & [ $0.593 , 0.604$ ] & -  \\    
        \fi
        \bottomrule
    \end{tabular}
    }
    \label{tab:fakeG_IE}
\end{table*}

\begin{table*}[!t]
    \centering
    \caption{
    %{\color{red} To update.}
    Comparing \textbf{\em interval estimate values} of Bias Mitigation Technique Imp-weighting}
\resizebox{14cm}{!}{
      \begin{tabular}{c  c @{\hspace{0.5em}} c @{\hspace{1em}} c @{\hspace{0.5em}} c @{\hspace{1em}} c @{\hspace{0.5em}} c}
        \toprule
        \multicolumn{7}{c}{\bf (A) Pseudo-Generator}\\
        \midrule
        \textbf{GT} & \multicolumn{2}{c}{\textbf{Baseline}\cite{choiFairGenerativeModeling2020a}}& \multicolumn{2}{c}{\textbf{Diversity}\cite{keswaniAuditingDiversityUsing2021}} & \multicolumn{2}{c}{\textbf{(Ours) CLEAM}}
        \\
         \cmidrule(lr){1-1}\cmidrule(lr){2-3}\cmidrule(lr){4-5} \cmidrule(lr){6-7}
        %Baseline
        % &P.Est($p^*_0$) & Error &I.Est.($p^*_0$) & Max Error
        &$\rho_{\texttt{Base}}(\pstar_0)$ & $e_\rho(\pstar_0)(\downarrow)$ 
         %Diversity
         %&P.Est.($p^*_0$) & Error &I.Est.($p^*_0$) & Max Error
         &$\rho_{\texttt{Div}}(\pstar_0)$ & $e_\rho(\pstar_0)(\downarrow)$ 
         %CLEAM
        %& P.Est.($p^*_0$) & Error & I.Est.($p^*_0$) & Max Error
        &$\rho_{\texttt{CLEAM}}{\texttt(\pstar_0)}$ & $e_\rho(\pstar_0)(\downarrow)$\\
        \toprule
        \multicolumn{7}{c}{\bf (B)   Importance Re-weighting \cite{choiFairGenerativeModeling2020a} GAN}\\
        \toprule
        \multicolumn{7}{c}{$\balpha$=[0.976,0.979], \texttt{Gender}}\\
        \midrule
        Unweighted & [$0.721  ,0.732 $] & - & [$0.697,0.722$] & - & [$0.733 ,0.744 $] & -  
        \\
        Weighted & [$0.674 ,0.685 $] & -  & [$0.658,0.684$] & - & [$0.686 ,0.693 $] & -\\
        \midrule
        \multicolumn{7}{c}{$\balpha$=[0.881,0.887], \texttt{BlackHair}}\\
         \midrule
        Unweighted & [$0.725 ,0.733 $] & - & [$0.704,0.729$] & -  & [$0.798 ,0.809 $] & -\\
        Weighted & [$0.710 ,0.722 $] & - & [$0.696,0.716$] & - & [$0.778 ,0.792 $] & -\\
        \iffalse
        \toprule
        \multicolumn{7}{c}{\bf (C)  MaGNET Sampling \cite{humayunMaGNETUniformSampling2021a} GAN}\\
        \toprule
        \multicolumn{7}{c}{$\balpha$=[0.976,0.979], \texttt{Gender}}\\
        \midrule
        $z$ & [$ 0.562 , 0.570 $] & - & [$0.555,0.575$] & - & [ $0.566 , 0.574$ ] & - \\
        $MaGNET(z)$  & [$0.516 , 0.525$] & - & [$0.515,0.535$] & - & [$0.519 , 0.528$ ] & - \\    
        \midrule
        \multicolumn{7}{c}{$\balpha$=[0.881,0.887], \texttt{BlackHair}}\\
        \midrule
        $z$ & [ $0.543 , 0.552$ ] & -  & [$0.540,0.560$] & - & $[ 0.560 , 0.572$ ] & -  \\
        $MaGNET(z)$ & [ $0.568 , 0.577$ ] & - &  [$0.560,0.590$] & - & [ $0.593 , 0.604$ ] & -  \\    
        \fi
        \bottomrule
    \end{tabular}
    }
    \label{tab:fakeG_IE}
\end{table*}

\section{More Bias Mitagation re-evaluation}
\subsection{More details evaluating Bias mitigation technique Imp-re-weighting}
\textcolor{red}{To Include training details such as Bias=90\_10 and perc=1.0}

\subsection{Evaluating Bias mitigation technique: MaGNET}
Similarly, we examine MaGNET\cite{humayunMaGNETUniformSampling2021a} a sampling algorithm that improves fairness, by enforcing uniformity on the latent feature space. We utilize the official code and weights in \cite{humayunMaGNETUniformSampling2021a} to generate both the original latent vector $z$ and the MaGNET latent vector, MaGNET($z$). We input these vectors into the StyleGAN2 provided by \cite{humayunMaGNETUniformSampling2021a}, trained on the FFHQ dataset \cite{karrasStyleBasedGeneratorArchitecture2019} to generate samples. Unlike the original implementation that applies Microsoft Cognitive API as the latent attribute classifier, we instead apply the same ResNet-18 model, for experimental consistency, therefore our results are slightly different from those in \cite{humayunMaGNETUniformSampling2021a}.
Regardless, we note that the original implementation also suffers from similar degrees of misclassification, as discussed in \cite{buolamwiniGenderShadesIntersectional2018}.
\begin{table*}[!t]
    \centering
    %New overall Caption
    \caption{
    {Point estimate of of bias mitigation techniques: MaGNET.}
    }
\resizebox{12.0cm}{!}{
      \begin{tabular}{c  @{\hspace{0.5em}} c @{\hspace{1em}} c @{\hspace{1em}} c }
        \toprule
          \textbf{Test} & \textbf{Baseline\cite{choiFairGenerativeModeling2020a}}& \textbf{Diversity}\cite{keswaniAuditingDiversityUsing2021} & \textbf{(Ours) CLEAM}
        \\
         \cmidrule(lr){1-1}\cmidrule(lr){2-2}\cmidrule(lr){3-3} \cmidrule(lr){4-4}
         %Baseline
        &$\mu_{\texttt{Base}}(\pstar_0)$
         %Diversity
        &$\mu_{\texttt{Div}}(\pstar_0)$
         %CLEAM
        &$\mu_{\texttt{CLEAM}}{\texttt(\pstar_0)}$ \\
        \iffalse
        \toprule
        \multicolumn{4}{c}{\bf (B) Importance Re-weighting \cite{choiFairGenerativeModeling2020a} GAN}\\
        \toprule
        \multicolumn{4}{c}{$\balpha$=[0.976,0.979], \texttt{Gender}}\\
        \midrule
        Unweighted & $0.727 $ & $0.723$ &  $0.738 $ \\
        Weighted & $0.711 $ & $0.710$   & $0.722 $ \\
        \midrule
        \multicolumn{4}{c}{$\balpha$=[0.881,0.887], \texttt{BlackHair}}\\
         \midrule
        Unweighted & $0.729 $  & $0.73$ & $0.803 $ \\
        Weighted & $0.716 $ & $0.72$ & $0.785 $ \\
        \toprule
        \fi
        \multicolumn{4}{c}{\bf (C) MaGNET Sampling \cite{humayunMaGNETUniformSampling2021a} GAN}\\
        \toprule
        \multicolumn{4}{c}{$\balpha$=[0.976,0.979], \texttt{Gender}}\\
        \midrule
        $z$ & $0.566$ & $0.565$ & $0.570$ \\
        $MaGNET(z)$ & $0.521$  & $0.525$  & $0.523$ \\    
        \midrule
        \multicolumn{4}{c}{$\balpha$=[0.881,0.887], \texttt{BlackHair}}\\
        \midrule
        $z$ & $0.547 $ & $0.550$ & $0.566$  \\
        $MaGNET(z)$  & $0.572$ & $0.575$  & $0.598$ \\
        \bottomrule
    \end{tabular}
    }
    \label{tab:biasMitigation_PE}
\end{table*}

\begin{table*}[!t]
    \centering
    \caption{
        {Interval estimate of of bias mitigation techniques: MaGNET.}}
\resizebox{14cm}{!}{
      \begin{tabular}{c  c @{\hspace{0.5em}} c @{\hspace{1em}} c @{\hspace{0.5em}} c @{\hspace{1em}} c @{\hspace{0.5em}} c}
        \toprule
        \multicolumn{7}{c}{\bf (C)  MaGNET Sampling \cite{humayunMaGNETUniformSampling2021a} GAN}\\
        \toprule
        \multicolumn{7}{c}{$\balpha$=[0.976,0.979], \texttt{Gender}}\\
        \midrule
        $z$ & [$ 0.562 , 0.570 $] & - & [$0.555,0.575$] & - & [ $0.566 , 0.574$ ] & - \\
        $MaGNET(z)$  & [$0.516 , 0.525$] & - & [$0.515,0.535$] & - & [$0.519 , 0.528$ ] & - \\    
        \midrule
        \multicolumn{7}{c}{$\balpha$=[0.881,0.887], \texttt{BlackHair}}\\
        \midrule
        $z$ & [ $0.543 , 0.552$ ] & -  & [$0.540,0.560$] & - & $[ 0.560 , 0.572$ ] & -  \\
        $MaGNET(z)$ & [ $0.568 , 0.577$ ] & - &  [$0.560,0.590$] & - & [ $0.593 , 0.604$ ] & -  \\    
        \bottomrule
    \end{tabular}
    }
%    \label{tab:fakeG_IE}
\end{table*}
